# Supplementary material for: Bounding and Estimating the Classical Information Rate of Quantum Channels with Memory
Source: arXiv:1903.00199 ancillary file (2020-02-17)
Supplement: Supplementary file 1 [file Addtional_Functions.pdf]

```
disp('This is the addition code.');
```

## Additional Functions

### Analog to Digital Quantization: A2D\_converter

```
function [ DiddalSig, thresholds ] = ...
    A2D_converter(AnalogSig, RANGE, number_of_state)
%Analog to digital convertor with uniformly speparated stages
% Output: 0~stagenumber-1
    if number_of_state < 2 || mod(number_of_state,1) ~= 0
        error('Please specify an integer >=2 as the number of stages.');
```

end

```
    constellation = RANGE(1):(RANGE(2)-RANGE(1))/(number_of_state-1):RANGE(2);
    DiddalSig = zeros(size(AnalogSig));
    for l = 1:numel(AnalogSig)
        [~,DiddalSig(l)] = min(abs(constellation - AnalogSig(l)));
    end
    DiddalSig = DiddalSig - 1;

    thresholds = zeros(1,number_of_state-1);
    for k = 1:number_of_state-1
        thresholds(k) = (constellation(k) + constellation(k+1))/2;
    end
end
```

### Decibel to Magnitude Converter: db2mag (

Decibel =  $10 \times \log_{10}(\text{Magnitude})$ )

```
function MAG = db2mag( DB )
    MAG = 10^(DB/10);
end
```

### Binary Input FIR Channel: BinaryInputFIRChannel

\* Requires suitable decimal-to-binary check-up table.

```
function [ Y, s ] = BinaryInputFIRChannel(G, snr, X, sp)
global de2biCheckUp
% Pass the binary input x through a FIR channel with input response
% coefficient (column) vector G, and SNR to be snr in dB.
% y is channle out put. s is next state

% We assume E[X^2] to be 1/2
%  $E[X^2] * \text{Sum}_k [g_k^2]$ 
% SNR =  $\frac{E[X^2] * \text{Sum}_k [g_k^2]}{E[Z^2]}$ 
%
%
% We treat 0 as -1, 1 as +1
%
%de2biCheckUp = ini_de2biCheckUp(numel(G)-1); % defined in file conf.m

if nargin < 4
```

```

    sp = 0; % By default, initialize the state to be zero.
end

sigma = sqrt(sum(G.^2)/(db2mag(snr))); % E[Z^2] = sigma^2
m = numel(G) - 1; % Memory
Y = zeros(size(X));
if m > 0
    for l = 1:numel(X)
        %u = [x, de2bi(sp,m)]; % = [X_l, X_{l-1}, ..., X_{l-m}]
        u = [X(l), de2biCheckUp(sp+1,:)];
        v = 2*u - 1;
        Y(l) = v*G + normrnd(0,sigma);
        sp = mod(2*sp+X(l),2^m);
    end
    s = sp;
else % Memoryless channel
    for l = 1:numel(X)
        Y(l) = (2*X(l)-1)*G + normrnd(0,sigma);
    end
    s = 0;
end
end
end

```

## Extracting the FSMC from the Binary Input FIR Channel: `firc2pmf`

```

function [ W ] = firc2pmf( G, sigma, thresholds, quantization)
% Generalize a FSMC  $W(s,p,y,x) = W(S=s, Y=y | S=p, X=x)$  w.r.t the binary
% impulse response channel specified with IR coefficient 'G', noise std. dev.
% 'sigma', quantization discriminator 'thresholds', and quantization level
% 'quantization'.
global de2biCheckUp
memory = numel(G)-1;
thres = [2*min(thresholds)-max(thresholds), ...
        thresholds,2*max(thresholds)-min(thresholds)];
matrix_W = zeros(2^memory, 2^memory, quantization, 2);
for i = 1:2
    x = i-1;
    for p = 1:2^memory
        u = 2*[x,de2biCheckUp(p,:)] - 1;
        % de2biCheckUp should match with G, reinitialization may be required
        mu = u*G;
        s = mod(2*(p-1)+x,2^memory) + 1;
        for y = 1:quantization
            interval = (thres(y+1)-thres(y))/100;
            T = thres(y):interval:thres(y+1);
            T = T(1:numel(T)-1);
            PDF = 1/sqrt(2*sigma^2*pi) * exp(-(T-mu).^2/(2*sigma^2));
            matrix_W(s,p,y,i) = sum(PDF)*interval;
        end
    end
end
W = cell(quantization, 2);
for y = 1:quantization
    for x = 1:2
        W{y,x} = sparse(matrix_W(:,:,y,x));
    end
end
end
end

```

## Generating a trivial Auxiliary FSMC: `trivial_conditional_pmf`

$\hat{W}^{y|x}(s|,s_p)$  is a uniform dstribution over  $y \in \mathcal{Y}$ , and  $s \in \mathcal{S}$  for any  $x$  and  $s_p$ .

```
function W = trivial_conditional_pmf(size_S, size_Y, size_X)
% Initialize a AF-FSMC W(s,p,y,x) = W(S=s, Y=y | S=p, X=x)
if nargin < 3
    size_X = 2;
end
if nargin < 2
    size_Y = 2;
end
if nargin < 1
    size_S = 2;
end
matrix_W = ones(size_S, size_S, size_Y, size_X)./(size_S * size_Y);
W = cell(size_Y, 2);
for y = 1:size_Y
    for x = 1:size_X
        W{y,x} = matrix_W(:,:,y,x);
    end
end
end
end
```

## Generating a random Auxiliary FSMC: `random_conditional_pmf`

For any  $x$  and  $s_p$ ,  $\hat{W}^{y|x}(s|,s_p)$  is chosen independently according to the *Haar* measure over the set of distributions over  $y$  and  $s$ .

```
function W = rand_conditional_pmf(size_S, size_Y, size_X)
% Initialize a AF-FSMC W(s,p,y,x) = W(S=s, Y=y | S=p, X=x)
if nargin < 3
    size_X = 2;
end
if nargin < 2
    size_Y = 2;
end
if nargin < 1
    size_S = 2;
end
matrix_W = rand(size_S, size_S, size_Y, size_X);
matrix_W = matrix_W./sum(matrix_W(:));
for x = 1:size_X
    for sp = 1:size_S
        A = matrix_W(:,sp,:,x);
        matrix_W(:,sp,:,x) = matrix_W(:,sp,:,x)./sum(A(:));
    end
end
W = cell(size_Y, 2);
for y = 1:size_Y
    for x = 1:size_X
        W{y,x} = matrix_W(:,:,y,x);
    end
end
end
end
```
