# Supplementary material for: Bounding and Estimating the Classical Information Rate of Quantum Channels with Memory
Source: arXiv:1903.00199 ancillary file (2020-02-17)
Supplement: Supplementary file 2 [file main_c.pdf]

## Binary FIR Channel: Estimating $I(W)$ , $\bar{I}(\hat{W})$ , $\underline{I}(\hat{W})$ , $\Delta(\hat{W})$ and

$$\frac{d}{dh} \Delta(\hat{W} + h \cdot D)$$

\*This script requires user defined function db2mag.m

\* The purpose of this script is to test the methodology on classical channels

```
clear;clc;
global de2biCheckUp
```

### Configuration

Number of channel usage in a row:

```
n = 1E6;
```

Impose response coefficient:

```
G = zeros(11,1);
for i = 1:11
    G(i) = 1/(1+(i-6)^2);
end
clear('i');
```

Gaussian Noise amplitude in dB (snr) and thus the std. dev. of the noise:

$$\sigma = \sqrt{\frac{\sum_i G_i^2}{\text{db2mag}(\text{snr})}}$$

```
snr = 5; %dB
sigma = sqrt(sum(G.^2)/(db2mag(snr))); %std. dev.
```

Quantization setup:

```
omax = 4*sqrt(sum(G.^2)/(db2mag(snr))) + sum(abs(G(:)));
omin = -omax;
quantization = 16; % which is the size of the output alphabet
```

Auxiliary channel memory size: #of state =  $2^{\text{memory}}$

```
memory = 2;
AF_num_of_states = 2^memory;
```

Amount of perturbation around the Auxiliary channel:

```
gamma = 1;
search_vec = (-1:0.05:1)*1e-3;
```

Print out the Configuration:

```
disp(['FIR Channel: G = ',mat2str(G,4)]);
disp(['SNR = ',num2str(snr),'dB.']);
disp(['Quantization configuration: ...', ...
      num2str(omin), '<---', num2str(quantization), '--->', num2str(omax)]);
```

### Initialization

```
rng('shuffle');
```

Store the decimal to binary string table for faster performance. We may have to reinitialize this table when the length of the binary input is different.

```
de2biCheckUp = zeros(2^(numel(G)-1),numel(G)-1);
for s = 1:1:2^(numel(G)-1)
    de2biCheckUp(s,:) = de2bi(s-1,numel(G)-1);
end
clear('s');
```

Preallocation:

```
lambda_y = ones(1,n);
lambda_x = ones(1,n);
lambda_xy = ones(1,n);
```

Other induced parameters:

```
dY = (omax - omin)/quantization;
num_of_states = 2^(numel(G)-1);
```

## Simulate Channle Input $X_1^n$ /Output $Y_1^n$ process

```
fprintf('Simulating channel with %d binary input ...', n);
X = randi(2,1,n)-1;
Y = BinaryInputFIRChannel(G, snr, X);
[Y, thresholds] = A2D_converter(Y, [omin,omax], quantization);
disp(' DONE.')
```

## Estimation of $\frac{1}{n} H(Y_1^n | X_1^n)$ using the following analytic method: (a numerical integration is involved)

Firstly, notice that:

$$P(Y_k | X_k, \dots, X_{k-m+1}) = \int_{\text{interval mapped to } Y_k} \frac{1}{\sqrt{2\sigma^2 \cdot \pi}} \cdot e^{-\frac{(t-\mu)^2}{2\sigma^2}} dt$$

where  $\sigma$  is the standard derivation of the involoved Gaussian noise, and  $\mu$  is the mean of the noise given  $X_{k-m+1}^k$ , namely

$$\mu := \sum_{i=1}^m X_{k-i+1} \cdot G_i.$$

Secondly, since  $\{Y_i\}_{i=1, \dots, n}$  are independent given  $X_1^n$ , we have

$$\frac{1}{n} H(Y_1^n | X_1^n) = \frac{1}{n} \sum_{i=1, \dots, n} H(Y_i | X_1^n).$$

Ignoring the effect of the initila state (or assuming the initial state is generated in a suitable random manner), and due to the fact that  $X_1^n$  are i.i.d., we have

$$\frac{1}{n} \sum_{i=1, \dots, n} H(Y_i | X_1^n) \approx H(Y_m | X_1^m),$$

which equals

$$-\sum_{\mathbf{x}_1^m} P_{\mathbf{x}_1^m}(\mathbf{x}_1^m) \cdot \sum_{y_m} P_{Y_m | \mathbf{x}_1^m}(\mathbf{x}_1^m, y_m) \cdot \log P_{Y_m | \mathbf{x}_1^m}(\mathbf{x}_1^m, y_m).$$

```
thres = [2*min(thresholds)-max(thresholds), ...
         thresholds, 2*max(thresholds)-min(thresholds)];
h = zeros(1,2^quantization);
k = 1;
for x = 0:1:2^numel(G)-1
    u = 2*de2bi(x,numel(G))-1;
    mu = u*G;
    P = zeros(1,quantization);
    for y = 1:quantization
        interval = (thres(y+1)-thres(y))/100;
        T = thres(y):interval:thres(y+1);
        T = T(1:numel(T)-1);
        PDF = 1/sqrt(2*sigma^2*pi) * exp(-(T-mu).^2/(2*sigma^2));
        P(y) = sum(PDF)*interval;
    end
    h(k) = -P*log2(P)';
    k = k + 1;
end
hY_given_X = sum(h)/2^numel(G);
clear('thres','h','k','u','mu','P','x','y','T','PDF','interval');
```

## (Optional) Using Forward Message Passing Method w.r.t the actual FSMC $W$ to estimate

$$\frac{1}{n} H(Y_1^n)$$

Abstract the actual FSMC in format of

$$W^{y|x}(s, s_p) = P(S_{l+1} = s, Y_l = y | S_l = s_p, X_l = x)$$

```
W = firc2pmf( G, sigma, thresholds, quantization);
```

$$Wq^{y|s}(s, s_p) := \sum_x Q(x) \cdot W^{y|x}(s, s_p)$$

```
Wq = cell(quantization,1);
```

```

for y = 1:quantization
    Wq{y} = (W{y,1}+W{y,2})/2; % Prob(s,y|p) = Sum_x Q(x)*Prob(s,y|p,x)
end

```

Initialize the state distribution  $\mu_0 = (1, 0, \dots, 0)$ :

```

mu = zeros(num_of_states,1);
mu(1) = 1;

```

Forward Pass:

$$\begin{aligned}\mu_l &= Wq^{Y_l-1} \cdot \overline{\mu_{l-1}}; \\ \lambda_l &:= |\mu_l|_1; \\ \overline{\mu}_l &= \mu_l / \lambda_l;\end{aligned}$$

```

for l = 1:n
    P = Wq{Y(l)+1};%squeeze(Wq(:,:,Y(l)+1));
    mu = P*mu;
    lambda_y(l) = sum(mu(:));
    mu = mu/lambda_y(l); % Normalize to get distribution of state at time l+1
end
clear('l','P','mu');

```

Estimate  $\frac{1}{n} H(Y^n) \approx -\frac{1}{n} \cdot \sum_{l=1}^n \log(\lambda_l)$ :

```

hY = -sum(log2(lambda_y))/n;

```

Information rate  $I := \frac{1}{n} I(X_1^n; Y_1^n) = \frac{1}{n} H(Y_1^n) - \frac{1}{n} H(Y_1^n | X_1^n)$ :

```

I = hY - hY_given_X;
disp(['Information Rate: ', num2str(I), ' bits per channel use.']);

```

## Setup an initial AF-FSMC $\widehat{W}$

Reinitialize the decimal to binary string table

```

de2biCheckUp = zeros(2^(memory),memory);
for s = 1:1:2^(memory)
    de2biCheckUp(s,:) = de2bi(s-1,memory);
end
clear('s');

```

Initialize a AF-FSMC  $\widehat{W}^{y|x}(s, s_p)$ ,  $\widehat{W}^y(s, s_p)$  in the same format. In this case we use a

1. uniform distribution;
2. or a random distribution generated via  $P(s, s_p, y, x) \propto \text{rand}(|\mathcal{S}|, |\mathcal{S}|, |\mathcal{Y}|, |\mathcal{X}|)$ ;
3. or the FSMC w.r.t. the partial response, in particular  $\widehat{G} := (G_1, \dots, G_{\text{memory}})$

```

fprintf('Initializing AF-FSMC ...');
W = rand_conditional_pmf(AF_num_of_states,quantization);
% or trivial_conditional_pmf(AF_num_of_states,quantization);
% or firc2pmf(G(1:memory+1), sigma, thresholds, quantization);
% or rand_conditional_pmf(AF_num_of_states,quantization);
Wq = cell(quantization,1);
for y = 1:quantization
    Wq{y} = (W{y,1}+W{y,2})/2;
end
clear('y');
disp(' DONE. ');

```

**BCJR estimation of  $\bar{I}(\widehat{W}) := \sum_{\mathbf{x}_1^n, \mathbf{y}_1^n} Q(\mathbf{x}_1^n) W(\mathbf{y}_1^n | \mathbf{x}_1^n) \log \left( \frac{W(\mathbf{y}_1^n | \mathbf{x}_1^n)}{Q\widehat{W}(\mathbf{y}_1^n)} \right)$**

Here  $Q\widehat{W}(\mathbf{y}_1^n) := \sum_{\mathbf{x}_1^n} Q(\mathbf{x}_1^n) \widehat{W}(\mathbf{y}_1^n)$ .

```

mu = zeros(AF_num_of_states,1);
mu(1) = 1;
fprintf('Run BCJR for H(Y) ...');
for l = 1:n
    P = Wq{Y(l)+1};%squeeze(Wq(:,:,Y(l)+1));
    mu = P*mu;
    lambda_y(l) = sum(mu(:));
end

```

```

mu = mu/lambda_y(l); % Normalize
end
clear('l','mu','P');
upper_hY = -sum(log2(lambda_y))/n;% + log2(dY);
fprintf(' DONE. ');
upper_bound = upper_hY - hY_given_X;
disp(['Initial upper bound: ',num2str(upper_bound), 'bits per channel use.']);

```

$$\text{BCJR Estimation of } \underline{I}(\widehat{W}) := \sum_{\mathbf{x}_1^n, \mathbf{y}_1^n} Q(\mathbf{x}_1^n) W(\mathbf{x}_1^n) \log \left( \frac{\widehat{W}(\mathbf{y}_1^n | \mathbf{x}_1^n)}{Q\widehat{W}(\mathbf{y}_1^n)} \right)$$

```

mu = zeros(AF_num_of_states,1);
mu(1) = 1;
fprintf('Run BCJR for H(Y|X) ...');
for l = 1:n
    P = W{Y(l)+1,X(l)+1};%squeeze(Wq(:,:,Y(l)+1));
    mu = P*mu;
    lambda_xy(l) = sum(mu(:));
    mu = mu/lambda_xy(l); % Normalize
end
clear('l','mu','P');
aux_hXY = -sum(log2(lambda_xy))/n;% + log2(dY);
fprintf(' DONE. ');
lower_bound = upper_hY - aux_hXY;
disp(['Initial lower bound: ',num2str(lower_bound), 'bits per channel use.']);

```

$$\text{Estimate } \Delta(\widehat{W}) := \bar{I}(\widehat{W}) - \underline{I}(\widehat{W})$$

Now, we are interested in computing the gap function defined above, or say,

$$\Delta(\widehat{W}) = \frac{1}{n} \sum_{\mathbf{x}_1^n, \mathbf{y}_1^n} W(\mathbf{x}_1^n, \mathbf{y}_1^n) \cdot \log \left( \frac{W(\mathbf{y}_1^n | \mathbf{x}_1^n)}{\widehat{W}(\mathbf{y}_1^n | \mathbf{x}_1^n)} \right)$$

```

gap = upper_bound - lower_bound;
disp(['Initial gap: ',num2str(gap), 'bits per channel use.']);

```

## Perturbating $\widehat{W}^{y|x}(s, s_p)$

### Basis of change

Note that

$$W^{y|x}(s, s_p) := P(S_{l+1} = s, Y_l = y | S_l = s_p, X_l = x).$$

Thus, define, for each  $(\check{x}, \check{s}_p) \in \mathcal{X} \times \mathcal{S}^*$ ,  $(\check{y}, \check{s}) \in \mathcal{Y} \times \mathcal{S} \setminus \{(0,0)\}$ , (we fix  $\gamma$  to be a suitable nonzero real number)

$$D[\check{s}, \check{y}, \check{s}_p, \check{x}] : (s, y, s_p, x) \mapsto \begin{cases} \gamma & \text{if } s = \check{s}, y = \check{y}, s_p = \check{s}_p, x = \check{x}, \\ -\gamma & \text{if } s = 0, y = 0, s_p = \check{s}_p, x = \check{x}, \\ 0 & \text{otherwise.} \end{cases}$$

We claim a basis of the tangent space of *the space of the FSMCs* at an interior point is given by

$$\beta := \{D[\check{s}, \check{y}, \check{s}_p, \check{x}]\}_{(\check{x}, \check{s}_p) \in \mathcal{X} \times \mathcal{S}^*, (\check{y}, \check{s}) \in \mathcal{Y} \times \mathcal{S} \setminus \{(0,0)\}}$$

```

BASIS_OF_CHANGE = cell(1,2*AF_num_of_states*(quantization*AF_num_of_states-1));
k = 0;
for cx = 1:2
    for csp = 1:AF_num_of_states
        for cy = 1:quantization
            for cs = 1:AF_num_of_states
                if cy ~= 1 || cs ~= 1
                    matrix_D = zeros(AF_num_of_states, AF_num_of_states, quantization, 2);
                    matrix_D(cs,csp,cy,cx) = gamma;
                    matrix_D(1,csp,1,cx) = -gamma;
                    D = cell(quantization, 2);
                    for y = 1:quantization
                        for x = 1:2
                            D{y,x} = matrix_D(:,:,y,x);
                        end
                    end
                    k = k+1;
                    BASIS_OF_CHANGE{k} = D;
                end
            end
        end
    end
end

```

```
end
clear('k','cx','csp','cy','cs','cy','matrix_D','D','y','x');
```

#### Pick a direction

We choose a random element in the span of the basis generated above.

```
D = cell(quantization, 2);
for y = 1:quantization
    for x = 1:2
        D{y,x} = zeros(AF_num_of_states);
    end
end
direction = rand(1,numel(BASIS_OF_CHANGE))-1;
for k = 1:numel(BASIS_OF_CHANGE)
    d = BASIS_OF_CHANGE{k};
    for y = 1:quantization
        for x = 1:2
            D{y,x} = D{y,x} + direction(k)*d{y,x};
        end
    end
end
clear('y','x','k','d');
```

**Walk along  $\hat{W} + h \cdot D$  (where  $h$  is in a neighbourhood of 0), and estimate  $\Delta(\hat{W} + h \cdot D)$**

Search range has already been defined in Line 17:

$$h \in \{-1, -0.95, -0.9, \dots, -0.05, 0, 0.05, \dots, 0.9, 0.95, 1\} \cdot 0.001$$

```
k = 0;
GAP = zeros(1,numel(search_vec));
```

For each  $h$ , prepare the AF-FSMC  $\hat{W} + h \cdot D$ , and run forward pass to estimate ?:

```
fprintf('Line search ... ');
for h = search_vec
```

prepare the AF-FSMC  $\hat{W} + h \cdot D$ :

```
new_W = cell(quantization,2);
for y = 1:quantization
    for x = 1:2
        new_W{y,x} = W{y,x} + h*D{y,x};
    end
end
new_Wq = cell(quantization,1);
for y = 1:quantization
    new_Wq{y} = (new_W{y,1}+new_W{y,2})/2;
end
```

Forward pass:

```
mu = zeros(AF_num_of_states,1);
mu(1) = 1;
for l = 1:n
    P = new_W{Y(l)+1,X(l)+1};
    mu = P*mu;
    lambda_xy(l) = sum(mu(:));
    mu = mu/lambda_xy(l);
end
clear('l','mu','P');
aux_hXY = -sum(log2(lambda_xy))/n;% + log2(dY);
gap = aux_hXY - hY_given_X;
k = k + 1;
GAP(k) = gap;
end
disp('DONE.');
```

Compute the derivative around  $\hat{W}$  empirically:

```
midpoint = (numel(search_vec)+1)/2; % We assume search_vec is of odd length
empirical_dev = (GAP(midpoint+1)-GAP(midpoint-1))/...
    (search_vec(midpoint+1)-search_vec(midpoint-1));
disp(['Empirical derivative along direction given by D is ', num2str(empirical_dev)]);
```

Plot the  $\Delta(\hat{W} + h \cdot D)$  for  $h$  in this range:

```
plot(search_vec,GAP);
```

```
clear('k', 'h', 'new_W', 'new_Wq', 'x', 'y', 'lambda_xy', 'aux_hXY', 'gap', 'midpoint');
```

## Alternative method to compute the (directional) derivative $\frac{d}{dh} \Delta(\widehat{W} + h \cdot D)$

By rewriting

$$\frac{d}{dh} \Delta(\widehat{W} + h \cdot D) = \frac{d}{dh} \frac{1}{n} \sum_{\mathbf{x}_1^n, \mathbf{y}_1^n} W(\mathbf{x}_1^n, \mathbf{y}_1^n) \cdot \log \left( \frac{W(\mathbf{y}_1^n | \mathbf{x}_1^n)}{(\widehat{W} + h \cdot D)(\mathbf{y}_1^n | \mathbf{x}_1^n)} \right) = -\frac{1}{n} \left\langle \frac{d}{dh} \log \left( (\widehat{W} + h \cdot D)(\mathbf{y}_1^n | \mathbf{x}_1^n) \right) \right\rangle_{W(\mathbf{x}_1^n, \mathbf{y}_1^n)},$$

and under some stationary/ergodicity assumption, we shall estimate

$$\frac{d}{dh} \Delta(\widehat{W} + h \cdot D) \approx -\frac{1}{n} \frac{d}{dh} \log \left( (\widehat{W} + h \cdot D)(\check{\mathbf{y}}_1^n | \check{\mathbf{x}}_1^n) \right)$$

where  $\check{\mathbf{x}}_1^n, \check{\mathbf{y}}_1^n$  are some *typical* input/output instances. Note that

$$(\widehat{W} + h \cdot D)(\check{\mathbf{y}}_1^n | \check{\mathbf{x}}_1^n) := \sum_{s_0^n} \prod_{l=1}^n (\widehat{W}^{\check{y}_l | \check{x}_l}(s_l, s_{l-1}) + h \cdot D^{\check{y}_l | \check{x}_l}(s_l, s_{l-1})) \cdot \mu^{(0)}(s_0)$$

where  $\mu^{(0)}$  is the *setup* of the initial channel state. Therefore,

$$\left. \frac{d}{dh} \right|_{h=0} \Delta(\widehat{W} + h \cdot D) \approx -\frac{1}{n} \cdot \log_2(e) \cdot \frac{\sum_{s_0^n} \sum_{k=1}^n \prod_{l \neq k} \widehat{W}^{\check{y}_l | \check{x}_l}(s_l, s_{l-1}) \cdot D^{\check{y}_k | \check{x}_k}(s_k, s_{k-1}) \cdot \mu^{(0)}(s_0)}{\widehat{W}(\check{\mathbf{y}}_1^n | \check{\mathbf{x}}_1^n)}.$$

Thus, if we define the messages (functions over  $\mathcal{S}^*$ )  $\{\mu^{(l)}\}_{l=0}^n$  and  $\{\nu^{(k)}\}_{k=0}^n$  (recursively) as

$$\mu^{(l)}(s_l) := \sum_{s_{l-1}} \widehat{W}^{\check{y}_l | \check{x}_l}(s_l, s_{l-1}) \cdot \mu^{(l-1)}(s_{l-1}) \quad \text{where } l = 1, 2, \dots, n;$$

```
MU = zeros(AF_num_of_states, n+1);
MU_balancer = ones(1, n+1);
MU(1, 1) = 1;
fprintf('Forward pass (for computing the dev) ...');
for l = 1:n
    P = W{Y(l)+1, X(l)+1};
    MU(:, l+1) = P*MU(:, l);
    MU_balancer(l+1) = sum(MU(:, l+1));
    MU(:, l+1) = MU(:, l+1) ./ MU_balancer(l+1);
end
disp('Done.');
```

$$\nu^{(k-1)}(s_{k-1}) := \sum_{s_k} \widehat{W}^{\check{y}_k | \check{x}_k}(s_k, s_{k-1}) \cdot \nu^{(k)}(s_k) \quad \text{where } k = n, n-1, \dots, 1;$$

```
NU = zeros(n+1, AF_num_of_states);
NU_balancer = ones(n+1, 1);
NU(n+1, :) = ones(1, AF_num_of_states);
fprintf('Backward pass (for computing the dev) ...');
for k = n:-1:1
    P = W{Y(k)+1, X(k)+1};
    NU(k, :) = NU(k+1, :)*P;
    NU_balancer(k) = sum(NU(k, :));
    NU(k, :) = NU(k, :)/NU_balancer(k);
end
disp('Done.');
```

where  $\mu^{(0)}$  has already been defined as the initial distribution of the channel state; whereas, we let  $\nu^{(n)}$  be the constant 1 function over  $s_n \in \mathcal{S}^*$ . In this case, we claim, for each  $k = 1, \dots, n$ ,

1.  $\sum_{s_0^n} \prod_{l \neq k} \widehat{W}^{\check{y}_l | \check{x}_l}(s_l, s_{l-1}) \cdot D^{\check{y}_k | \check{x}_k}(s_k, s_{k-1}) \cdot \mu^{(0)}(s_0) = \sum_{s_k, s_{k-1}} \nu^{(k)}(s_k) \cdot D^{\check{y}_k | \check{x}_k}(s_k, s_{k-1}) \cdot \mu^{(k-1)}(s_{k-1}) =: \langle \nu^{(k)} | D^{\check{y}_k | \check{x}_k} | \mu^{(k-1)} \rangle;$
2.  $\widehat{W}(\check{\mathbf{y}}_1^n | \check{\mathbf{x}}_1^n) = \sum_{s_0^n} \prod_{l=1}^n \widehat{W}^{\check{y}_l | \check{x}_l}(s_l, s_{l-1}) \cdot \mu^{(0)}(s_0) = \sum_{s_k} \nu^{(k)}(s_k) \cdot \mu^{(k)}(s_k) =: \langle \nu^{(k)} | \mu^{(k)} \rangle;$
3. Additionally,  $\widehat{W}(\check{\mathbf{y}}_1^n | \check{\mathbf{x}}_1^n) = \langle \nu^{(k)} | \widehat{W}^{\check{y}_k | \check{x}_k} | \mu^{(k-1)} \rangle.$

This enables us to write

$$\left. \frac{d}{dh} \right|_{h=0} \Delta(\widehat{W} + h \cdot D) \approx -\frac{1}{n} \cdot \log_2(e) \cdot \sum_{k=1}^n \frac{\langle \nu^{(k)} | D^{\check{y}_k | \check{x}_k} | \mu^{(k-1)} \rangle}{\langle \nu^{(k)} | \mu^{(k)} \rangle}.$$

Or, better off, we have

$$\text{Above} = -\frac{1}{n} \cdot \log_2(e) \cdot \sum_{k=1}^n \frac{\langle \mathcal{L}^{(k)} | D^{\hat{y}_k | \hat{x}_k} | \mu^{(k-1)} \rangle}{\langle \mathcal{L}^{(k)} | \hat{W}^{\hat{y}_k | \hat{x}_k} | \mu^{(k-1)} \rangle} = -\frac{1}{n} \cdot \log_2(e) \cdot \sum_{k=1}^n \frac{\langle \bar{\mathcal{L}}^{(k)} | D^{\hat{y}_k | \hat{x}_k} | \bar{\mu}^{(k-1)} \rangle}{\langle \bar{\mathcal{L}}^{(k)} | \bar{W}^{\hat{y}_k | \hat{x}_k} | \bar{\mu}^{(k-1)} \rangle}.$$

```

estimated_dev = 0;
for k = 1:n
    %P = W{Y(k)+1,X(k)+1};
    Q = D{Y(k)+1,X(k)+1};
    %estimated_dev = estimated_dev + (NU(k+1,:)*Q*MU(:,k))/(NU(k+1,:)*P*MU(:,k));
    estimated_dev = estimated_dev + (NU(k+1,:)*Q*MU(:,k))/(NU(k+1,:)*MU(:,k+1)*MU_balancer(k+1));
end
estimated_dev = -estimated_dev/n*log2(exp(1));
disp(['Estimated derivative alone direction given by D is ', num2str(estimated_dev)]);
clear('k','P','Q');

```

## Compute the gradient

We compute the gradient as

$$\nabla \Delta(\hat{W}) := \left( \frac{d}{dh} \Big|_{h=0} \Delta(\hat{W} + h \cdot D) \right)_{D \in \beta},$$

where we use either of the above two method to compute the involved directional derivative.

```

fprintf('Compute the gradient ... \n');
h = search_vec(2) - search_vec(1);
empirical_grad = zeros(size(BASIS_OF_CHANGE));
estimated_grad = zeros(size(BASIS_OF_CHANGE));

```

Prepare the messages:

Forward Pass:

```

MU = zeros(AF_num_of_states,n+1);
MU_balancer = ones(1,n+1);
MU(1,1) = 1;
for l = 1:n
    P = W{Y(l)+1,X(l)+1};
    MU(:,l+1) = P*MU(:,l);
    MU_balancer(l+1) = sum(MU(:,l+1));
    MU(:,l+1) = MU(:,l+1)./MU_balancer(l+1);
end
clear('P','l');

```

Backward Pass:

```

NU = zeros(n+1,AF_num_of_states);
NU_balancer = ones(n+1,1);
NU(n+1,:) = ones(1,AF_num_of_states);
for k = n:-1:1
    P = W{Y(k)+1,X(k)+1};
    NU(k,:) = NU(k+1,:)*P;
    NU_balancer(k) = sum(NU(k,:));
    NU(k,:) = NU(k,:)./NU_balancer(k);
end
clear('P','k');

```

Compute the gradient:

```

for b = 1:numel(BASIS_OF_CHANGE)
    D = BASIS_OF_CHANGE{b};

```

Empirical Method:

Evaluate  $\Delta(\hat{W} + h \cdot D)$ :

```

new_W = cell(quantization,2);
for y = 1:quantization
    for x = 1:2
        new_W{y,x} = W{y,x} + h*D{y,x};
    end
end
new_Wq = cell(quantization,1);
for y = 1:quantization
    new_Wq{y} = (new_W{y,1}+new_W{y,2})/2;
end
mu = zeros(AF_num_of_states,1);
mu(1) = 1;
for l = 1:n

```

```

P = new_W{Y(l)+1,X(l)+1};
mu = P*mu;
lambda_xy(l) = sum(mu(:));
mu = mu/lambda_xy(l);
end
clear('l','mu','P');
aux_hXY = -sum(log2(lambda_xy))/n;% + log2(dY);
gap_r = aux_hXY - hY_given_X;

```

Evaluate  $\Delta(\hat{W} - h \cdot D)$ :

```

new_W = cell(quantization,2);
for y = 1:quantization
    for x = 1:2
        new_W{y,x} = W{y,x} - h*D{y,x};
    end
end
new_Wq = cell(quantization,1);
for y = 1:quantization
    new_Wq{y} = (new_W{y,1}+new_W{y,2})/2;
end
mu = zeros(AF_num_of_states,1);
mu(1) = 1;
for l = 1:n
    P = new_W{Y(l)+1,X(l)+1};
    mu = P*mu;
    lambda_xy(l) = sum(mu(:));
    mu = mu/lambda_xy(l);
end
clear('l','mu','P');
aux_hXY = -sum(log2(lambda_xy))/n;% + log2(dY);
gap_l = aux_hXY - hY_given_X;

```

Compute  $\frac{\Delta(\hat{W} + h \cdot D) - \Delta(\hat{W} - h \cdot D)}{2h}$ :

```

empirical_grad(b) = (gap_r-gap_l)/(2*h);

```

Alternative method:

Combine the messages:

```

for k = 1:n
    %P = W{Y(k)+1,X(k)+1};
    Q = D{Y(k)+1,X(k)+1};
    %estimated_grad(b) = estimated_grad(b) + (NU(k+1,:)*Q*MU(:,k))/(NU(k+1,:)*P*MU(:,k));
    estimated_grad(b) = estimated_grad(b) + (NU(k+1,:)*Q*MU(:,k))/(NU(k+1,:)*MU(:,k+1)*MU_balancer(k+1));
end
estimated_grad(b) = -estimated_grad(b)/n*log2(exp(1));
clear('k','P','Q');

```

Compare the partial derivative:

```

fprintf('%d: %1.12f, %1.12f\n',b,empirical_grad(b),estimated_grad(b));
end
disp('Done.')

```

## Verification

Firstly, let's compare the gradient computed via the two methods:

```

fprintf('Norm(empirical_grad) = %f\n',norm(empirical_grad));
fprintf('Norm(estimated_grad) = %f\n',norm(estimated_grad));

```

Note that

$$\cos(\text{angle between two } \nabla\text{s}) = \frac{\langle \nabla_{EM} | \nabla_{ES} \rangle}{|\nabla_{EM}| \cdot |\nabla_{ES}|}$$

we can check whether the two gradients align with each other:

```

fprintf('cos(angle) = %f',dot(empirical_grad,estimated_grad)/(norm(empirical_grad)*norm(estimated_grad)))

```

We further can verify the result by comparing  $\frac{d}{dh} \Delta(\hat{W} + h \cdot D)$  with  $\sum_i d_i \cdot (\nabla \Delta(\hat{W}))_i$ :

```

empirical_dev_induced = 0;
for k = 1: numel(BASIS_OF_CHANGE)
    empirical_dev_induced = empirical_dev_induced + direction(k) * empirical_grad(k);
end

```

```
fprintf('empirical_dev = %f and <dir|estimated_grad> = %f\n', empirical_dev, empirical_dev_induced);
estimated_dev_induced = 0;
for k = 1:numel(BASIS_OF_CHANGE)
    estimated_dev_induced = estimated_dev_induced + direction(k) * estimated_grad(k);
end
fprintf('estimated_dev = %f and <dir|estimated_grad> = %f\n', estimated_dev, estimated_dev_induced);
clear('k');
```

### Save the result to a file

```
save(['main_c(', char(datetime('now', 'Format', 'yyyy-MM-dd''T''HHmmss')), ').mat']);
```
