# Supplementary material for: Bounding and Estimating the Classical Information Rate of Quantum Channels with Memory
Source: arXiv:1903.00199 ancillary file (2020-02-17)
Supplement: Supplementary file 3 [file main_cgd.pdf]

# Classical FSMCs: Optimizing $\Delta(\hat{W})$ using modified gradient descent algorithm

\*This script requires user defined function db2mag.m

\*In this script, we propose an algorithm in minimizing  $\Delta(\hat{W})$ . This algorithm is based on:

1. The idea of the gradient descent algorithm
2. The 'alternative' method in estimating the directional derivative as listed in main\_c.mlx.

However, computing the derivative as in step '2' is of complexity  $O(n)$ ; as a result, computing the gradient using '2' would take  $O(n \cdot (|\mathcal{X}| \cdot |\mathcal{S}| \cdot (|\mathcal{Y}| \cdot |\mathcal{S}| - 1)))$  number of steps, which is required in each gradient descent iteration. In the algorithm presented below, we managed to develop a work around, and reduce the complexity of each gradient descent iteration to  $O(n)$ !

```
clear;clc;
global de2biCheckUp
```

## Configuration

Number of channel usage in a row:

```
n = 5E6;
```

Impose response coefficient:

```
G = zeros(11,1);
for i = 1:11
    G(i) = 1/(1+(i-6)^2);
end
clear('i');
G = [0.5;1;0.5];
```

Gaussian Noise amplitude in dB (snr) and thus the std. dev. of the noise:

$$\sigma = \sqrt{\frac{\sum_i G_i^2}{\text{db2mag}(\text{snr})}}$$

```
snr = 5; %dB
sigma = sqrt(sum(G.^2)/(db2mag(snr))); %std. dev.
```

Quantization setup:

```
omax = 4*sqrt(sum(G.^2)/(db2mag(snr))) + sum(abs(G(:)));
omin = -omax;
quantization = 16; % which is the size of the output alphabet
```

Auxiliary channel memory size: #of state =  $2^{\text{memory}}$

```
memory = 2;
AF_num_of_states = 2^memory;
```

Step size and the limit on the number of steps in the gradient descent algorithm:

```
gamma = 0.01;
gd_limit = 50;
```

Step limit of the iterative expectation?maximization (EM) algorithm

```
em_limit = 50;
```

Print out the Configuration:

```
disp(['FIR Channel: G = ',mat2str(G,4)]);
disp(['SNR = ',num2str(snr),'dB.']);
disp(['Quantization configuration: ...', ...
    num2str(omin), '<---', num2str(quantization),'--->', num2str(omax)]);
```

## Initialization

```
rng('shuffle');
```

Store the decimal to binary string table for faster performance. We may have to reinitialize this table when the length of the binary input is different.

```
de2biCheckUp = zeros(2^(numel(G)-1),numel(G)-1);
for s = 1:1:2^(numel(G)-1)
    de2biCheckUp(s,:) = de2bi(s-1,numel(G)-1);
end
clear('s');
```

Preallocation:

```
lambda_y = ones(1,n);
lambda_x = ones(1,n);
lambda_xy = ones(1,n);
```

Other induced parameters:

```
dY = (omax - omin)/quantization;
num_of_states = 2^(numel(G)-1);
```

## Simulate Channle Input $X_1^n$ /Output $Y_1^n$ process

```
fprintf('Simulating channel with %d binary input ...', n);
X = randi(2,1,n)-1;
Y = BinaryInputFIRChannel(G, snr, X);
[Y, thresholds] = A2D_converter(Y,[omin,omax],quantization);
disp(' DONE.')
```

## Estimation of $\frac{1}{n} H(Y_1^n | X_1^n)$ using the following analytic method: (a numerical integration is involved)

Firstly, notice that:

$$P(Y_k | X_k, \dots, X_{k-m+1}) = \int_{\text{interval mapped to } Y_k} \frac{1}{\sqrt{2\sigma^2 \cdot \pi}} \cdot e^{-\frac{(t-\mu)^2}{2\sigma^2}} dt$$

where  $\sigma$  is the standard derivation of the involoved Gaussian noise, and  $\mu$  is the mean of the noise given  $X_{k-m+1}^k$ , namely

$$\mu := \sum_{i=1}^m X_{k-i+1} \cdot G_i.$$

Secondly, since  $\{Y_l\}_{l=1, \dots, n}$  are independent given  $X_1^n$ , we have

$$\frac{1}{n} H(Y_1^n | X_1^n) = \frac{1}{n} \sum_{l=1, \dots, n} H(Y_l | X_1^n).$$

Ignoring the effect of the initila state (or assuming the initial state is generated in a suitable random manner), and due to the fact that  $X_1^n$  are i.i.d., we have

$$\frac{1}{n} \sum_{l=1, \dots, n} H(Y_l | X_1^n) \approx H(Y_m | X_1^m),$$

which equals

$$-\sum_{\mathbf{x}_1^m} P_{X_1^m}(\mathbf{x}_1^m) \cdot \sum_{y_m} P_{Y_m | X_1^m, \dots, x_1}(y_m) \cdot \log P_{Y_m | X_1^m, \dots, x_1}(y_m).$$

```
thres = [2*min(thresholds)-max(thresholds), ...
         thresholds, 2*max(thresholds)-min(thresholds)];
h = zeros(1,2^quantization);
k = 1;
for x = 0:1:2^numel(G)-1
    u = 2*de2bi(x,numel(G))-1;
    mu = u*G;
    P = zeros(1,quantization);
    for y = 1:quantization
        interval = (thres(y+1)-thres(y))/100;
        T = thres(y):interval:thres(y+1);
        T = T(1:numel(T)-1);
        PDF = 1/sqrt(2*sigma^2*pi) * exp(-(T-mu).^2/(2*sigma^2));
        P(y) = sum(PDF)*interval;
    end
    h(k) = -P*log2(P)';
    k = k + 1;
end
hY_given_X = sum(h)/2^numel(G);
clear('thres','h','k','u','mu','P','x','y','T','PDF','interval');
```

## Maximum value of $\Delta(\hat{W})$

$$\Delta(\hat{W}) = \frac{1}{n} \cdot \hat{H}(Y_1^n | X_1^n) - \frac{1}{n} \cdot H(Y_1^n | X_1^n) \leq \frac{1}{n} \cdot \hat{H}(Y_1^n) - \frac{1}{n} \cdot H(Y_1^n | X_1^n) \leq \frac{1}{n} \cdot \log_2(|\mathcal{Y}|) - \frac{1}{n} \cdot H(Y_1^n | X_1^n)$$

```
GAP_MAX = log2(quantization) - hY_given_X;
```

## (Optional) Using Forward Message Passing Method w.r.t the actual FSMC $W$ to estimate $\frac{1}{n} H(Y_1^n)$

Abstract the actual FSMC in format of

$$W^{y|x}(s, s_p) = P(S_{t+1} = s, Y_t = y | S_t = s_p, X_t = x)$$

```
W = firc2pmf( G, sigma, thresholds, quantization);
```

$$Wq^{y}(s, s_p) := \sum_x Q(x) \cdot W^{y|x}(s, s_p)$$

```
Wq = cell(quantization,1);
for y = 1:quantization
    Wq{y} = (W{y,1}+W{y,2})/2; % Prob(s,y|p) = Sum_x Q(x)*Prob(s,y|p,x)
end
```

Initilize the state distribution  $\mu_0 = (1, 0, \dots, 0)$ :

```
mu = zeros(num_of_states,1);
```

```
mu(1) = 1;
```

Forward Pass:

$$\begin{aligned}\mu_l &= Wq^{Y_{l-1}} \cdot \overline{\mu}_{l-1}; \\ \lambda_l &:= |\mu_l|_1; \\ \overline{\mu}_l &= \mu_l / \lambda_l;\end{aligned}$$

```
for l = 1:n
    P = Wq{Y(l)+1};%squeeze(Wq(:, :, Y(l)+1));
    mu = P*mu;
    lambda_y(l) = sum(mu(:));
    mu = mu/lambda_y(l); % Normalize to get distribution of state at time l+1
end
clear('l', 'P', 'mu');
```

Estimate  $\frac{1}{n} H(Y_1^n) \approx -\frac{1}{n} \cdot \sum_{l=1}^n \log(\lambda_l)$ :

```
hY = -sum(log2(lambda_y))/n;
```

Information rate  $I := \frac{1}{n} I(X_1^n; Y_1^n) = \frac{1}{n} H(Y_1^n) - \frac{1}{n} H(Y_1^n | X_1^n)$ :

```
I = hY - hY_given_X;
disp(['Information Rate: ', num2str(I), ' bits per channel use.']);
```

## Setup an initial AF-FSMC $\widehat{W}$

Reinitialize the decimal to binary string table

```
de2biCheckUp = zeros(2^(memory), memory);
for s = 1:1:2^(memory)
    de2biCheckUp(s, :) = de2bi(s-1, memory);
end
clear('s');
```

Initialize a AF-FSMC  $\widehat{W}^{y|x}(s, s_p)$ ,  $\widehat{W}q^y(s, s_p)$  in the same format. In this case we use a

1. uniform distribution;
2. or a random distribution generated via  $P(s, s_p, y, x) \propto \text{rand}(|\mathcal{S}|, |\mathcal{S}|, |\mathcal{Y}|, |\mathcal{X}|)$ ;
3. or the FSMC w.r.t. the partial response, in particular  $\widehat{G} := (G_1, \dots, G_{\text{memory}})$

```
fprintf('Initializing AF-FSMC ...');
W = firc2pmf(G(1:memory+1), sigma, thresholds, quantization);
% or trivial_conditional_pmf(AF_num_of_states, quantization);
% or firc2pmf(G(1:memory+1), sigma, thresholds, quantization);
% or rand_conditional_pmf(AF_num_of_states, quantization);
Wq = cell(quantization, 1);
for y = 1:quantization
    Wq{y} = (W{y, 1} + W{y, 2}) / 2;
end
clear('y');
disp(' DONE.');
```

## Gradient Descent Method

```
gd_time = zeros(1, gd_limit+1);
gd_time(1) = 0;
gd_W_List = cell(1, gd_limit+1);
gd_W_List{1} = W;
```

Using the 'alternaive' method developed in `main_c.mlx`, we know the gradient of  $\Delta(\widehat{W})$  can be estimated via

$$\begin{aligned}\nabla \Delta(\widehat{W}) &= \sum_{D \in \beta} \frac{d}{dh} \Big|_{h=0} \Delta(\widehat{W} + h \cdot D) \cdot D \\ \frac{d}{dh} \Big|_{h=0} \Delta(\widehat{W} + h \cdot D) &\approx -\frac{1}{n} \cdot \log_2(e) \cdot \sum_{k=1}^n \frac{\langle \underline{\nu}^{(k)} | D^{\tilde{y}_k \tilde{x}_k} | \underline{\mu}^{(k-1)} \rangle}{\langle \underline{\nu}^{(k)} | \widehat{W}^{\tilde{y}_k \tilde{x}_k} | \underline{\mu}^{(k-1)} \rangle} = -\frac{1}{n} \cdot \log_2(e) \cdot \sum_{k=1}^n \frac{\langle \underline{\nu}^{(k)} | D^{\tilde{y}_k \tilde{x}_k} | \underline{\mu}^{(k-1)} \rangle}{\langle \underline{\nu}^{(k)} | \widehat{W}_i^{\tilde{y}_k \tilde{x}_k} | \underline{\mu}^{(k-1)} \rangle},\end{aligned}$$

where  $\underline{\nu}$  is some *orthonormal* basis of the tangent space (around  $\widehat{W}$ ), and the messages (functions over  $\mathcal{S}^*$ )  $\{\underline{\mu}^{(l)}\}_{l=0}^n$ ,  $\{\underline{\nu}^{(k)}\}_{k=0}^n$  and thier normalized version  $\{\overline{\mu}^{(l)}\}_{l=0}^n$ ,  $\{\overline{\nu}^{(k)}\}_{k=0}^n$  can be computed recursively through forward message passing and backward message passing, respectively. (For details about the definition of these messages, please refer to `main_c.mlx`.) Therefore, for each gradient descent iteration, we need to carry out the update as follows (say the gradient descent coefficient is 1):

$$\widehat{W}_{t+1} \leftarrow \widehat{W}_t - \sum_{D \in \beta} \frac{d}{dh} \Big|_{h=0} \Delta(\widehat{W}_t + h \cdot D) \cdot D \approx \widehat{W}_t + \frac{1}{n} \cdot \log_2(e) \cdot \sum_{D \in \beta} \sum_{k=1}^n \frac{\langle \underline{\nu}^{(k)} | D^{\tilde{y}_k \tilde{x}_k} | \overline{\mu}^{(k-1)} \rangle}{\langle \underline{\nu}^{(k)} | \widehat{W}_t^{\tilde{y}_k \tilde{x}_k} | \overline{\mu}^{(k-1)} \rangle} \cdot D.$$

There are two problems with above update rule:

1. It is computational heavy as pointed out in the beginning of this document. In particular, it is  $|\beta|$  times slower than (Sadeghi, Vontobel and Shams, 2009).
2. Unless we somehow choose  $\beta$  based on  $\widehat{W}_t$  carefully, there is always a possibility that  $\widehat{W}_{t+1}$  may no long be a valid FSMC by involoving negative entries. This means, a *projection* will be needed in every iteration. Such a '*projection*' can be a LP, a CVX or an analytical solution.

**To solve problem 1:**

For an *interior* AF-FSMC  $\hat{W}$ , its tangent space  $\mathcal{T}$  is a subspace of all real-valued functions, namely

$$\mathcal{T} = \left\{ D : \mathcal{X} \times \mathcal{Y} \times \mathcal{S}^* \times \mathcal{S}^* \rightarrow \mathbf{R} \mid \sum_{y,s} D(x, y, s, s_p) = 0 \quad \forall (x, s_p) \in \mathcal{X} \times \mathcal{S}^* \right\},$$

where  $\mathcal{B}$  is an *orthonormal* basis for  $\mathcal{T}$ . Now, suppose we extend  $\mathcal{B}$  into an orthonormal basis  $\mathcal{F}$  of  $\mathcal{T} = \{ D : \mathcal{X} \times \mathcal{Y} \times \mathcal{S}^* \times \mathcal{S}^* \rightarrow \mathbf{R} \}$ , and define

$$\nabla_{\mathcal{F}} \Delta(\hat{W}) := \sum_{A \in \alpha} \frac{d}{dh} \Big|_{h=0} \Delta(\hat{W} + h \cdot A) \cdot A.$$

We make following assertions:

1.  $\nabla_{\mathcal{F}} \Delta(\hat{W}) - \nabla \Delta(\hat{W})$  is orthomormal to all the vectors in  $\mathcal{T}$ , and thus orthomormal to  $\mathcal{T}$ . On other words,  $\nabla \Delta(\hat{W})$  is the *projection* of  $\nabla_{\mathcal{F}} \Delta(\hat{W})$  onto the subspace  $\mathcal{T}$ .

Proof: By writing  $\nabla_{\mathcal{F}} \Delta(\hat{W}) - \nabla \Delta(\hat{W})$  as a linear combination of the vectors in  $\alpha \setminus \beta$ , we are done.

2.  $\nabla_{\mathcal{F}} \Delta(\hat{W})$  does not depend on  $\mathcal{B}$ , as long as the basis  $\mathcal{B}$  is orthonormal.

Proof: or any other orthonormal basis  $\alpha' = \{\alpha'_1, \dots, \alpha'_M\}$ , there must exist some orthonormal matrix  $U$  s.t.  $[\alpha'_1, \dots, \alpha'_M]^T = U \cdot [\alpha_1, \dots, \alpha_M]^T$ ; thus

$$\begin{aligned} \sum_i \frac{d}{dh} \Big|_{h=0} \Delta(\hat{W} + h \cdot \alpha'_i) \cdot \alpha'_i &= \sum_i \left( \sum_j U_{i,j} \cdot \frac{d}{dh} \Big|_{h=0} \Delta(\hat{W} + h \cdot \alpha_j) \right) \cdot \left( \sum_k U_{i,k} \cdot \alpha_k \right) \\ &= \sum_{j,k} \left( \sum_i U_{i,j} \cdot U_{i,k} \right) \cdot \frac{d}{dh} \Big|_{h=0} \Delta(\hat{W} + h \cdot \alpha_j) \cdot \alpha_k \\ &= \sum_{j,k} \delta_{j,k} \cdot \frac{d}{dh} \Big|_{h=0} \Delta(\hat{W} + h \cdot \alpha_j) \cdot \alpha_k = \nabla_{\mathcal{F}} \Delta(\hat{W}). \end{aligned}$$

As a result, by utilizing the standard orthonormal basis of  $\mathcal{T}$ , namely,  $\{ e_{\hat{x}, \hat{y}, \hat{s}, \hat{s}_p} : (x, y, s, s_p) \mapsto \delta_{x, \hat{x}} \cdot \delta_{y, \hat{y}} \cdot \delta_{s, \hat{s}} \cdot \delta_{s_p, \hat{s}_p} \}_{\hat{x}, \hat{y}, \hat{s}, \hat{s}_p}$ , we can estimate  $\nabla_{\mathcal{F}} \Delta(\hat{W})$  as

$$\nabla_{\mathcal{F}} \Delta(\hat{W}) \approx -\frac{1}{n} \cdot \log_2(e) \cdot \sum_{\hat{x}, \hat{y}, \hat{s}, \hat{s}_p} \sum_{k=1}^n \frac{\langle \bar{\nu}^{(k)} | e_{\hat{x}, \hat{y}, \hat{s}, \hat{s}_p} | \bar{\mu}^{(k-1)} \rangle}{\langle \bar{\nu}^{(k)} | \hat{W}_r^{\hat{y}_k \hat{s}_k | \hat{s}_k | \bar{\mu}^{(k-1)} \rangle} \cdot e_{\hat{x}, \hat{y}, \hat{s}, \hat{s}_p} = -\frac{1}{n} \cdot \log_2(e) \cdot \sum_{k=1}^n \frac{|\bar{\mu}^{(k-1)} \rangle \langle \bar{\nu}^{(k)} |}{\langle \bar{\nu}^{(k)} | \hat{W}_r^{\hat{y}_k \hat{s}_k | \hat{s}_k | \bar{\mu}^{(k-1)} \rangle}$$

which can be computed in  $O(n)!$  On the other hand, projection of  $\nabla_{\mathcal{F}} \Delta(\hat{W})$  onto the subspace  $\mathcal{T}$  is fairly easy, since a *orthogonal* basis of the orthogonal subspace of  $\mathcal{T}$  is given by

$$\{(x, y, s, s_p) \mapsto \delta_{x, \hat{x}} \cdot \delta_{y, \hat{y}} \cdot \delta_{s, \hat{s}} \cdot \delta_{s_p, \hat{s}_p}\}_{\hat{x}, \hat{y}, \hat{s}, \hat{s}_p}.$$

**IN SUMMARY**, above described a method in computing the gradient in  $O(n + M)$ :

```
tic;
f = waitbar(0, 'The gradient method ... ');
for gd_counter = 1:gd_limit
```

**1. Messaging passing;**

```
% Forward pass
waitbar((gd_counter-1)/gd_limit, f, ...
    sprintf('%d Forward pass ... ', gd_counter));
MU = zeros(AF_num_of_states, n+1);
MU_balancer = ones(1, n+1);
MU(1, 1) = 1;
for l = 1:n
    P = W{Y(l)+1, X(l)+1};
    MU(:, l+1) = P * MU(:, l);
    MU_balancer(l+1) = sum(MU(:, l+1));
    MU(:, l+1) = MU(:, l+1) ./ MU_balancer(l+1);
end
clear('P', 'l');
% Backward pass
waitbar((gd_counter-0.75)/gd_limit, f, ...
    sprintf('%d Backward pass ... ', gd_counter));
NU = zeros(n+1, AF_num_of_states);
NU_balancer = ones(n+1, 1);
NU(n+1, :) = ones(1, AF_num_of_states);
for k = n:-1:1
    P = W{Y(k)+1, X(k)+1};
    NU(k, :) = NU(k+1, :) * P;
    NU_balancer(k) = sum(NU(k, :));
    NU(k, :) = NU(k, :) ./ NU_balancer(k);
end
clear('P', 'k');
```

**2. Estimate  $\nabla_{\mathcal{F}} \Delta(\hat{W})$  as  $-\frac{1}{n} \cdot \log_2(e) \cdot \sum_{k=1}^n \frac{|\bar{\mu}^{(k-1)} \rangle \langle \bar{\nu}^{(k)} |}{\langle \bar{\nu}^{(k)} | \hat{W}_r^{\hat{y}_k \hat{s}_k | \hat{s}_k | \bar{\mu}^{(k-1)} \rangle}$ :**

```
waitbar((gd_counter-0.5)/gd_limit, f, ...
    sprintf('%d Estimate gradient ... ', gd_counter));
estimated_grad = cell(quantization, 2);
for x = 1:2
    for y = 1:quantization
        estimated_grad{y, x} = zeros(AF_num_of_states);
    end
end
clear('x', 'y');
```

```

temp = -log2(exp(1))/n;
for k = 1:n
    estimated_grad{Y(k)+1,X(k)+1} = estimated_grad{Y(k)+1,X(k)+1} + ...
        temp*(transpose(NU(k+1,:))*ttranspose(MU(:,k)))/(NU(k+1,:)*MU(:,k+1)*MU_balancer(k+1));
end
clear('temp','k');

```

3. Project  $\nabla_{\mathcal{F}} \Delta(\hat{W})$  onto the subspace  $\mathcal{S}$  by eliminating its components w.r.t.  $\{(x, y, s, s_p) \mapsto \delta_{x,\hat{x}} \cdot \delta_{s_p,\hat{s}_p}\}_{\hat{x},\hat{s}_p}$  one by one (in any order).

Actually, this step is redundant, given that we can solve [problem 2](#) as in next paragraph.

```

waitbar((gd_counter-0.25)/gd_limit,f,...
    sprintf('%d] Project onto the tangent space ... ', gd_counter));
for x = 1:2
    for sp = 1:AF_num_of_states
        Prob_SY = zeros(AF_num_of_states,quantization);
        for y = 1:quantization
            Prob_SY(:,y) = estimated_grad{y,x}(:,sp);
        end
        Prob_SY = Prob_SY - sum(Prob_SY(:))/(numel(Prob_SY));
        for y = 1:quantization
            estimated_grad{y,x}(:,sp) = Prob_SY(:,y);
        end
    end
end
clear('x','y','Prob_SY','sp');

```

### To solve problem 2:

Once an 'overshot' occurs, i.e., negative entries appear after descent along the (negative) gradient, an *intuitive*\* solution would be to project it back to the nearest point in the polyhedron of FSMCs. Namely,

$$\begin{aligned}
 & \min |\hat{W}_{t+1} - \lambda \cdot (\hat{W}_t - \nabla(\hat{W}_t))| \\
 & \text{s.t.} \quad \hat{W}_{t+1}^{y|x}(s|s_p) \geq 0 \quad \forall x, y, s, s_p \\
 & \quad \quad \sum_{y,s} \hat{W}_{t+1}^{y|x}(s|s_p) = 1 \quad \forall x, s_p
 \end{aligned}$$

This is a quadratic programming problem, and can be solved using `quadprog`\*\*.

Adaptive step size: I am still thinking about it. There are a number of choices:

1. Decaying as time goes; (Advantage: Easy to implement)
2. Linear w.r.t. the distance to the target; (Advantage: Guaranteed converges in a neighbourhood of the optimal point; Disadvantage: Too slow when approaching the target, and may be too unstable when far away from the target)
3. Get smaller as approaching the target, but in a non-linear fashion, e.g. a scale and shifted version of arctan. (Advantage: advantages of 2 while possibly avoiding its disadvantages; Disadvantage: You need to pick appropriate scaling and shifting factors, which can be tricky.)

```

waitbar((gd_counter-0.2)/gd_limit,f,...
    sprintf('%d] Gradient descent ... ', gd_counter));
for x = 1:2
    for y = 1:quantization
        W{y,x} = W{y,x} - gamma*estimated_grad{y,x};
    end
end
waitbar((gd_counter-0.15)/gd_limit,f,...
    sprintf('%d] Project to the nearest FSMC ... ', gd_counter));
DIS = 0;
for x = 1:2
    for sp = 1:AF_num_of_states
        Prob_SY = zeros(AF_num_of_states,quantization);
        for y = 1:quantization
            Prob_SY(:,y) = W{y,x}(:,sp);
        end
        [Prob_SY,dis] = nearest_prob(Prob_SY);
        DIS = DIS + dis^2;
        for y = 1:quantization
            W{y,x}(:,sp) = Prob_SY(:,y);
        end
    end
end
fprintf('%d] Projection distance = %f\n', gd_counter, sqrt(DIS));
clear('x','y','sp','Prob_SY','dis','DIS');

```

\*To justify such intuition informally, one may consider  $\hat{W}$  to be a boundary point of the FSMC-polytope, and the gradient is pointing 'outward' of the boundary. Then the best direction  $\hat{W}$  may take must lie on the boundary subspace. Therefore, one should consider the projection of the gradient onto this subspace, which is equivalent to solving the aforementioned optimization problem.

\*\*Indeed, if we replace the cost function with L1 norm, it can be easily solved as a linear programming. However, THIS WON'T WORK HERE, since L1 minimization favors the corner points, i.e., the FSMCs whose conditional probability contains a number of zeros. This is really detrimental in this application, since we may unwantedly end up with a FSMC whose output probability at a certain  $y$  is zero, which will yield a  $+\infty$  contribution to the  $\mathcal{F}$  function.

```

gd_W_List{gd_counter+1} = W;
gd_time{gd_counter+1} = toc;
end
close(f);
clear('gd_counter','f');

```

## Post processing for the GDA

For each  $\hat{W}$ , estimate  $\frac{1}{n}H(Y^n)$ , and compute  $\bar{I}(\hat{W})$ ,  $\underline{I}(\hat{W})$  and  $\Delta(\hat{W})$ .

```
fprintf('Gathering the data for the gradient descent method ... ');
f = waitbar(0,'Post-processing for the gradient method ... ');
gd_upper_hY_List = zeros(1,gd_limit);
gd_aux_hXY_List = zeros(1,gd_limit);
for gd_counter = 1:gd_limit+1
    W = gd_W_List{gd_counter};
    Wq = cell(quantization,1);
    for y = 1:quantization
        Wq{y} = (W{y,1}+W{y,2})/2;
    end
    % 1/n*H(Y1,...,Yn)
    mu = zeros(AF_num_of_states,1);
    mu(1) = 1;
    for l = 1:n
        P = Wq{Y(l)+1};
        mu = P*mu;
        lambda_y(l) = sum(mu(:));
        mu = mu/lambda_y(l);
    end
    cclear('l','mu','P');
    gd_upper_hY_List(gd_counter) = -sum(log2(lambda_y))/n;
    % 1/n*H(Y1,...,Yn|X1,...,Xn)
    mu = zeros(AF_num_of_states,1);
    mu(1) = 1;
    for l = 1:n
        P = W{Y(l)+1,X(l)+1};
        mu = P*mu;
        lambda_xy(l) = sum(mu(:));
        mu = mu/lambda_xy(l);
    end
    cclear('l','mu','P');
    gd_aux_hXY_List(gd_counter) = -sum(log2(lambda_xy))/n;
    waitbar(gd_counter/(gd_limit+1),f);
end
close(f);
clear('f','gd_counter');
gd_IR_L = gd_upper_hY_List - gd_aux_hXY_List;
gd_IR_U = gd_upper_hY_List - hY_given_X;
gd_GAP = gd_IR_U - gd_IR_L;
disp('Done.');
```

## Iterative expectation?maximization (EM) algorithm

```
em_time = zeros(1,em_limit+1);
em_time(1) = 0;
em_W_List = cell(1,em_limit+1);
em_W_List{1} = gd_W_List{1};
W = em_W_List{1};
tic;
f = waitbar(0,'The Iterative expectation?maximization (EM) algorithm ... ');
for em_counter = 1:em_limit
    % Forward pass
    %fprintf('[%d] Forward Pass ... ',em_counter);
    waitbar((em_counter-1)/gd_limit,f,...
        sprintf('[%d] Forward Pass ... ', em_counter));
    MU = zeros(AF_num_of_states,n+1);
    MU_balancer = ones(1,n+1);
    MU(1,1) = 1;
    for l = 1:n
        P = W{Y(l)+1,X(l)+1};
        MU(:,l+1) = P*MU(:,l);
        MU(:,l+1) = MU(:,l+1)./sum(MU(:,l+1));
    end
    cclear('P','l');
    % Backward pass
    %fprintf('Backward Pass ... ');
    waitbar((em_counter-0.7)/gd_limit,f,...
        sprintf('[%d] Backward Pass ... ', em_counter));
    NU = zeros(n+1,AF_num_of_states);
    NU_balancer = ones(n+1,1);
    NU(n+1,:) = ones(1,AF_num_of_states);
    for k = n:-1:1
        P = W{Y(k)+1,X(k)+1};
        NU(k,:) = NU(k+1,:)*P;
        NU(k,:) = NU(k,:)./sum(NU(k,:));
    end
    cclear('P','k');
    % Take statistical Average
    %fprintf('Combining ... ');
    waitbar((em_counter-0.4)/gd_limit,f,...
        sprintf('[%d] Combining the messages ... ', em_counter));
    next_W = cell(quantization,2);
```

```

for x = 1:2
    for y = 1:quantization
        next_W{y,x} = zeros(AF_num_of_states);
    end
end
clear('x','y');
for k = 1:n
    local_stat = (transpose(NU(k+1,:))*transpose(MU(:,k))).*W{Y(k)+1,X(k)+1};
    next_W{Y(k)+1,X(k)+1} = next_W{Y(k)+1,X(k)+1} + ...
        local_stat/(n*sum(local_stat(:)));
end
clear('k','local_stat');
% Properly normalize next_W
waitbar((em_counter-0.1)/gd_limit,f,...
    sprintf('[%d] Normalization ... ', em_counter));
for x = 1:2
    for sp = 1:AF_num_of_states
        Prob_SY = zeros(AF_num_of_states,quantization);
        for y = 1:quantization
            Prob_SY(:,y) = next_W{y,x}(:,sp);
        end
        Prob_SY = Prob_SY./sum(Prob_SY(:));
        for y = 1:quantization
            next_W{y,x}(:,sp) = Prob_SY(:,y);
        end
    end
end
W = next_W;
clear('next_W');
% Save it
em_W_List{em_counter+1} = W;
em_time(em_counter+1) = toc;
end
close(f);
clear('em_counter','f');

```

## Post processing for the EMA

For each  $\hat{W}$ , estimate  $\frac{1}{n}H(Y^n)$ , and compute  $\bar{I}(\hat{W})$ ,  $\underline{I}(\hat{W})$  and  $\Delta(\hat{W})$ .

```

fprintf('Gathering the data for the EM algorithm ... ');
f = waitbar(0,'Post-processing for the EM algorithm ... ');
em_upper_hY_List = zeros(1,em_limit);
em_aux_hXY_List = zeros(1,em_limit);
for em_counter = 1:em_limit+1
    W = em_W_List{em_counter};
    Wq = cell(quantization,1);
    for y = 1:quantization
        Wq{y} = (W{y,1}+W{y,2})/2;
    end
    % 1/n*H(Y1,...,Yn)
    mu = zeros(AF_num_of_states,1);
    mu(1) = 1;
    for l = 1:n
        P = Wq{Y(l)+1};
        mu = P*mu;
        lambda_y(l) = sum(mu(:));
        mu = mu/lambda_y(l);
    end
    clear('l','mu','P');
    em_upper_hY_List(em_counter) = -sum(log2(lambda_y))/n;
    % 1/n*H(Y1,...,Yn|X1,...,Xn)
    mu = zeros(AF_num_of_states,1);
    mu(1) = 1;
    for l = 1:n
        P = W{Y(l)+1,X(l)+1};
        mu = P*mu;
        lambda_xy(l) = sum(mu(:));
        mu = mu/lambda_xy(l);
    end
    clear('l','mu','P');
    em_aux_hXY_List(em_counter) = -sum(log2(lambda_xy))/n;
    waitbar(em_counter/(em_limit+1),f);
end
close(f);
clear('f','em_counter');
em_IR_L = em_upper_hY_List - em_aux_hXY_List;
em_IR_U = em_upper_hY_List - hY_given_X;
em_GAP = em_IR_U - em_IR_L;
disp('Done. ');

```

## Plot

```

hold on;
plot(gd_time,gd_IR_L,'b');
plot(gd_time,gd_IR_U,'r');
plot(em_time,em_IR_L,'b--');

```

```
plot(em_time,em_IR_U,'r--');
plot([0,max([gd_time,em_time])],ones(1,2)*I,'k--');
hold off;
legend('GD:IRLB','GD:IRUB','EM:IRLB','EM:IRUB','IR');
title(sprintf('Gradient Descent Method with "QP drag-back" in each step\n and Iterative expectation?maximization algorithm
xlabel('Time/seconds');
ylabel('bits/channel use');
xlim([0,gd_time(gd_limit+1)]);
```

### Save the result to a file

```
save(['main_cgd(',char(datetime('now','Format','yyyy-MM-dd'T'HHmmss)),')mat']);
```
