# Supplementary material for: Bounding and Estimating the Classical Information Rate of Quantum Channels with Memory
Source: arXiv:1903.00199 ancillary file (2020-02-17)
Supplement: Supplementary file 4 [file main_q.pdf]

# Quantum-State Channels: Estimating $I(W)$ , $\bar{I}(\hat{W})$ , $\underline{I}(\hat{W})$ , $\Delta(\hat{W})$ and $\frac{d}{dh} \Delta(\hat{W} + h \cdot D)$

\*This script aims to migrate and verify the method in estimating  $\frac{d}{dh} \Delta(\hat{W} + h \cdot D)$  in FSMC case to the case of QSCs.

```
clear;clc;rng('shuffle');
```

## Configuration

# of consecutive channel usage to be simulated:

```
n = 1e5;
```

# of qubits in the memory/state system, the principle/input/output system, and the environment system:

```
sdim = 2;  
pdim = 2;  
envdim = 2;
```

Input distribution

```
Q = ones(1,2^pdim);  
Q = Q./sum(Q(:));
```

Amount of perturbation around the Auxiliary channel:

```
search_vec = (-1:0.05:1)*1e-1;
```

## Initialization

Standard Classical-to-Quantum modulation:

$$x \mapsto |x\rangle\langle x|.$$

```
C2Q = cell(1,2^pdim);  
for x = 1:2^pdim  
    temp = zeros(2^pdim,1);  
    temp(x) = 1;  
    C2Q{x} = temp;  
end  
clear('x','temp');
```

Standard partial measurement setup:

$$M_y := I_S \otimes |y\rangle\langle y|.$$

```
M = cell(1,2^pdim);  
for y = 1:2^pdim  
    temp = zeros(2^pdim);  
    temp(y,y) = 1;  
    M{y} = tensor(eye(2^sdim),temp);  
end  
clear('y','temp');
```

Generate a random quantum-state channel:

```
W = matrix_QSC(unitary2Qop( randU(2^(pdim+sdim+envdim)),envdim),C2Q,M);  
QW = cell(2^pdim,1);  
for y = 1:2^pdim  
    temp = zeros(size(W{1}));  
    for x = 1:2^pdim  
        temp = temp + W{y,x}.*Q(x);  
    end  
    QW{y} = temp;  
end  
clear('x','y','temp');
```

Preallocation:

```
lambda_y = ones(1,n);  
lambda_x = ones(1,n);  
lambda_xy = ones(1,n);
```

## Simulate Channle Input $X_1^n$ /Output $Y_1^n$ process

```
fprintf('Simulating channel with %d binary i/o ... ', n);  
X = randi(2,1,n)-1;  
Y = zeros(size(X));  
rho = eye(2^sdim)/2^sdim; rho = rho(:);  
one = eye(2^sdim); one = one(:);  
L = transpose(tril(ones(2^pdim)));  
for k = 1:n  
    PMF = zeros(1,2^pdim);  
    for y = 1:2^pdim
```

```

        PMF(y) = dot(W{y,X(k)+1}*rho,one);
    end
    CDF = PMF*L;
    Y(k) = sum(rand > CDF);
    rho = W{Y(k)+1,X(k)+1}*rho;
    rho = rho./dot(one,rho);
end
disp('Done. ');
clear('rho','one','PMF','CDF','L','k','y');

```

Using Forward Message Passing Method w.r.t the actual QSC  $W$  to estimate  $\frac{1}{n} H(Y_1^n | X_1^n)$

```

fprintf('Estimating H(Y|X) ... ');
rho = eye(2^sdim)/2^sdim; rho = rho(:);
one = eye(2^sdim); one = one(:);
for k = 1:n
    rho = W{Y(k)+1,X(k)+1}*rho;
    lambda_xy(k) = dot(one,rho);
    rho = rho./lambda_xy(k);
end
hY_given_X = -sum(log2(lambda_xy))/n;
fprintf(' = %f\n', hY_given_X);
clear('rho','one','k');

```

Using Forward Message Passing Method w.r.t the actual QSC  $W$  to estimate  $\frac{1}{n} H(Y_1^n)$

```

fprintf('Estimating H(Y) ... ');
rho = eye(2^sdim)/2^sdim; rho = rho(:);
one = eye(2^sdim); one = one(:);
for k = 1:n
    rho = QW{Y(k)+1}*rho;
    lambda_y(k) = dot(one,rho);
    rho = rho./lambda_y(k);
end
hY = -sum(log2(lambda_y))/n;
fprintf(' = %f\n', hY);
clear('rho','one','k');

```

### Information Rate

```

I = hY - hY_given_X;
fprintf('Information rate = %f\n', I);

```

### Setup an initial AF-QSC $\hat{W}$

We simply re-generate another random QSC:

```

W = matrix_QSC(unitary2Qop( randU(2^(pdim+sdim+envdim)),envdim),C2Q,M);
QW = cell(2^pdim,1);
for y = 1:2^pdim
    temp = zeros(size(W{1}));
    for x = 1:2^pdim
        temp = temp + W{y,x}.*Q(x);
    end
    QW{y} = temp;
end
clear('x','y','temp');

```

Using Forward Message Passing Method w.r.t the AF-QSC  $\hat{W}$  to estimate  $\frac{1}{n} H(Y_1^n | X_1^n)$

```

fprintf('Estimating auxiliary H(Y|X) ... ');
rho = eye(2^sdim)/2^sdim; rho = rho(:);
one = eye(2^sdim); one = one(:);
for k = 1:n
    rho = W{Y(k)+1,X(k)+1}*rho;
    lambda_xy(k) = dot(one,rho);
    rho = rho./lambda_xy(k);
end
aux_hXY = -sum(log2(lambda_xy))/n;
fprintf(' = %f\n', aux_hXY);
clear('rho','one','k');

```

Using Forward Message Passing Method w.r.t the AF-QSC  $\hat{W}$  to estimate  $\frac{1}{n} H(Y_1^n)$

```

fprintf('Estimating upper bound for H(Y) ... ');
rho = eye(2^sdim)/2^sdim; rho = rho(:);
one = eye(2^sdim); one = one(:);
for k = 1:n
    rho = QW{Y(k)+1}*rho;

```

```

lambda_y(k) = dot(one, rho);
rho = rho./lambda_y(k);
end
upper_hY = -sum(log2(lambda_y))/n;
fprintf(' = %f\n', upper_hY);
clear('rho', 'one', 'k');

```

## Information Rate Upper/Lower bounds and the gap

```

fprintf('Information rate upper bound = %f\n', upper_hY - hY_given_X);
fprintf('Information rate lower bound = %f\n', upper_hY - aux_hXY);
fprintf('Gap = %f\n', aux_hXY - hY_given_X);

```

## Perturbating $\hat{W}^{y|x}(s, \bar{s}; s_p, \bar{s}_p)$

Let's go the easy way: We regenerate a QSC and consider the difference:

```

fprintf('Generating a direction in the tangent space ... ');
Wt = matrix_QSC(unitary2Qop( randU(2^(pdim+sdim+envdim)), envdim), C2Q, M);
D = cell(2^pdim, 2^pdim);
for y = 1:2^pdim
    for x = 1:2^pdim
        D{y,x} = Wt{y,x} - W{y,x};
    end
end
clear('x', 'y');
disp('Done. ');

```

## Walking along the direction $D$

```

k = 0;
GAP = zeros(1, numel(search_vec));

```

For each  $h$ , prepare the QSC  $\hat{W} + h \cdot D$ , and run forward pass to estimate ?:

```

fprintf('Line search ... ');
for h = search_vec

```

prepare the AF-FSMC  $\hat{W} + h \cdot D$ :

```

new_W = cell(2^pdim, 2^pdim);
for y = 1:2^pdim
    for x = 1:2^pdim
        new_W{y,x} = W{y,x} + h*D{y,x};
    end
end
new_Wq = cell(2^pdim, 1);
for y = 1:2^pdim
    new_Wq{y} = zeros(4^sdim);
    for x = 1:2^pdim
        new_Wq{y} = new_Wq{y} + new_W{y,x}.*Q(x);
    end
end

```

Forward pass:

```

rho = eye(2^sdim)/2^sdim; rho = rho(:);
one = eye(2^sdim); one = one(:);
for l = 1:n
    rho = new_W{Y(l)+1, X(l)+1}*rho;
    lambda_xy(l) = dot(one, rho);
    rho = rho./lambda_xy(l);
end
aux_hXY = -sum(log2(lambda_xy))/n;
clear('rho', 'one', 'l');
gap = aux_hXY - hY_given_X;
k = k + 1;
GAP(k) = gap;
fprintf('\nGAP(%d) = %f', k, gap);
end
disp('DONE. ');

```

Compute the derivative around  $\hat{W}$  empirically:

```

midpoint = (numel(search_vec)+1)/2; % We assume search_vec is of odd length
empirical_dev = (GAP(midpoint+1)-GAP(midpoint-1))/...
    (search_vec(midpoint+1)-search_vec(midpoint-1));
disp(['Empirical derivative along direction given by D is ', num2str(empirical_dev)]);

```

Plot the  $\Delta(\hat{W} + h \cdot D)$  for  $h$  in this range:

```

plot(search_vec, GAP);
clear('k', 'h', 'new_W', 'new_Wq', 'x', 'y', 'lambda_xy', 'aux_hXY', 'gap', 'midpoint');

```

Alternative method to compute the (directional) derivative  $\frac{d}{dh} \Delta(\hat{W} + h \cdot D)$

By rewriting

$$\frac{d}{dh} \Delta(\widehat{W} + h \cdot D) = \frac{d}{dh} \frac{1}{n} \sum_{\mathbf{x}_1^n, \mathbf{y}_1^n} W(\mathbf{x}_1^n, \mathbf{y}_1^n) \cdot \log \left( \frac{W(\mathbf{y}_1^n | \mathbf{x}_1^n)}{(\widehat{W} + h \cdot D)(\mathbf{y}_1^n | \mathbf{x}_1^n)} \right) = -\frac{1}{n} \left\langle \frac{d}{dh} \log \left( (\widehat{W} + h \cdot D)(\mathbf{y}_1^n | \mathbf{x}_1^n) \right) \right\rangle_{W(\mathbf{x}_1^n, \mathbf{y}_1^n)},$$

and under some stationary/ergodicity assumption, we shall estimate

$$\frac{d}{dh} \Delta(\widehat{W} + h \cdot D) \approx -\frac{1}{n} \frac{d}{dh} \log \left( (\widehat{W} + h \cdot D)(\check{\mathbf{y}}_1^n | \check{\mathbf{x}}_1^n) \right)$$

where  $\check{\mathbf{x}}_1^n, \check{\mathbf{y}}_1^n$  are some *typical* input/output instances. Note that

$$(\widehat{W} + h \cdot D)(\check{\mathbf{y}}_1^n | \check{\mathbf{x}}_1^n) := \sum_{s_0, \bar{s}_0} \delta(s_n, \bar{s}_n) \cdot \prod_{l=1}^n (\widehat{W}^{\check{y}_l \check{x}_l}(s_l, \bar{s}_l; s_{l-1}, \bar{s}_{l-1}) + h \cdot D^{\check{y}_l \check{x}_l}(s_l, \bar{s}_l; s_{l-1}, \bar{s}_{l-1})) \cdot \rho^{(0)}(s_0, \bar{s}_0)$$

where  $\rho^{(0)}$  is the density operator of the initial channel state. Therefore,

$$\left. \frac{d}{dh} \right|_{h=0} \Delta(\widehat{W} + h \cdot D) \approx -\frac{1}{n} \cdot \log_2(e) \cdot \frac{\sum_{s_0, \bar{s}_0} \delta(s_n, \bar{s}_n) \cdot \sum_{k=1}^n \prod_{l \neq k} \widehat{W}^{\check{y}_l \check{x}_l}(s_l, \bar{s}_l; s_{l-1}, \bar{s}_{l-1}) \cdot D^{\check{y}_k \check{x}_k}(s_k, \bar{s}_k; s_{k-1}, \bar{s}_{k-1}) \cdot \rho^{(0)}(s_0, \bar{s}_0)}{\widehat{W}(\check{\mathbf{y}}_1^n | \check{\mathbf{x}}_1^n)}.$$

Thus, if we define the messages (PSD operators over  $\mathcal{H}_S$ )  $\{\rho^{(l)}\}_{l=0}^n$  and  $\{\sigma^{(k)}\}_{k=0}^n$  (recursively) as

$$\rho^{(l)}(s_l, \bar{s}_l) := \sum_{s_{l-1}, \bar{s}_{l-1}} \widehat{W}^{\check{y}_l \check{x}_l}(s_l, \bar{s}_l; s_{l-1}, \bar{s}_{l-1}) \cdot \rho^{(l-1)}(s_{l-1}, \bar{s}_{l-1}) \quad \text{where } l = 1, 2, \dots, n;$$

```
fprintf('Forward pass ... ');
rho = eye(2^sdim)/2^sdim;
RHO = zeros(4^sdim, n+1);
RHO(:, 1) = rho(:);
RHO_balancer = ones(1, n+1);
one = eye(2^sdim); one = one(:);
for k = 1:n
    RHO(:, k+1) = W{Y(k)+1, X(k)+1}*RHO(:, k);
    RHO_balancer(k+1) = dot(one, RHO(:, k+1));
    RHO(:, k+1) = RHO(:, k+1)./RHO_balancer(k+1);
end
clear('rho', 'k', 'one');
```

$$\sigma^{(k-1)}(s_{k-1}, \bar{s}_{k-1}) := \sum_{s_k, \bar{s}_k} \widehat{W}^{\check{y}_k \check{x}_k}(s_k, \bar{s}_k; s_{k-1}, \bar{s}_{k-1}) \cdot \sigma^{(k)}(s_k, \bar{s}_k) \quad \text{where } k = n, n-1, \dots, 1;$$

```
fprintf('Backward pass ... ');
sigma = eye(2^sdim);
rSIGMA = zeros(4^sdim, n+1);
rSIGMA(:, 1) = sigma(:);
rSIGMA_balancer = ones(1, n+1);
one = eye(2^sdim); one = one(:);
trans_W = cell(size(W));
for k = 1:numel(W)
    trans_W{k} = transpose(W{k});
end
for k = 1:n
    rSIGMA(:, k+1) = trans_W{Y(n-k+1)+1, X(n-k+1)+1}*rSIGMA(:, k);
    rSIGMA_balancer(k+1) = dot(one, rSIGMA(:, k+1));
    rSIGMA(:, k+1) = rSIGMA(:, k+1)./rSIGMA_balancer(k+1);
end
SIGMA = zeros(n+1, 4^sdim);
SIGMA_balancer = ones(n+1, 1);
for k = 1:n+1
    SIGMA(k, :) = transpose(rSIGMA(:, n+2-k));
    SIGMA_balancer(k) = rSIGMA_balancer(n+2-k);
end
clear('trans_W', 'sigma', 'k', 'one', 'rSIGMA', 'rSIGMA_balancer');
```

where  $\rho^{(0)}$  has already been defined as the initial density operator of the channel state; whereas, we let  $\sigma^{(n)}$  be the identity operator over  $\mathcal{H}_S$ . In this case, we claim, for each  $k = 1, \dots, n$ ,

1.  $\sum_{s_0, \bar{s}_0} \delta(s_n, \bar{s}_n) \cdot \prod_{l \neq k} \widehat{W}^{\check{y}_l \check{x}_l}(s_l, \bar{s}_l; s_{l-1}, \bar{s}_{l-1}) \cdot D^{\check{y}_k \check{x}_k}(s_k, \bar{s}_k; s_{k-1}, \bar{s}_{k-1}) \cdot \rho^{(0)}(s_0, \bar{s}_0) = \sum_{s_k, \bar{s}_k} \sigma^{(k)}(s_k, \bar{s}_k) \cdot D^{\check{y}_k \check{x}_k}(s_k, \bar{s}_k; s_{k-1}, \bar{s}_{k-1}) \cdot \rho^{(k-1)}(s_{k-1}, \bar{s}_{k-1}) =: \langle \sigma^{(k)} | D^{\check{y}_k \check{x}_k} | \rho^{(k-1)} \rangle$ ;
2.  $\widehat{W}(\check{\mathbf{y}}_1^n | \check{\mathbf{x}}_1^n) = \sum_{s_0, \bar{s}_0} \prod_{l=1}^n \widehat{W}^{\check{y}_l \check{x}_l}(s_l, \bar{s}_l; s_{l-1}, \bar{s}_{l-1}) \cdot \rho^{(0)}(s_0, \bar{s}_0) = \sum_{s_k, \bar{s}_k} \sigma^{(k)}(s_k, \bar{s}_k) \cdot \rho^{(k)}(s_k, \bar{s}_k) =: \langle \sigma^{(k)} | \rho^{(k)} \rangle$ ;
3. Additionally,  $\widehat{W}(\check{\mathbf{y}}_1^n | \check{\mathbf{x}}_1^n) = \langle \sigma^{(k)} | \widehat{W}^{\check{y}_k \check{x}_k} | \rho^{(k-1)} \rangle$ .

This enables us to write

$$\left. \frac{d}{dh} \right|_{h=0} \Delta(\widehat{W} + h \cdot D) \approx -\frac{1}{n} \cdot \log_2(e) \cdot \sum_{k=1}^n \frac{\langle \sigma^{(k)} | D^{\check{y}_k \check{x}_k} | \rho^{(k-1)} \rangle}{\langle \sigma^{(k)} | \rho^{(k)} \rangle}.$$

Or, better off, we have

$$\text{Above} = -\frac{1}{n} \cdot \log_2(e) \cdot \sum_{k=1}^n \frac{\langle \sigma^{(k)} | \widehat{W}^{\check{y}_k \check{x}_k} | \rho^{(k-1)} \rangle}{\langle \sigma^{(k)} | \widehat{W}^{\check{y}_k \check{x}_k} | \rho^{(k-1)} \rangle} = -\frac{1}{n} \cdot \log_2(e) \cdot \sum_{k=1}^n \frac{\langle \sigma^{(k)} | D^{\check{y}_k \check{x}_k} | \rho^{(k-1)} \rangle}{\langle \sigma^{(k)} | \widehat{W}^{\check{y}_k \check{x}_k} | \rho^{(k-1)} \rangle}.$$

```

fprintf('Estimating the derivative ');
estimated_dev = 0;
for k = 1:n
    T = D{Y(k)+1,X(k)+1};
    estimated_dev = estimated_dev + (SIGMA(k+1,:)*T*RHO(:,k))/(SIGMA(k+1,:)*RHO(:,k+1)*RHO_balancer(k+1));
end
estimated_dev = -estimated_dev/n*log2(exp(1));
disp(['= ', num2str(estimated_dev)]);
clear('T','k');

```

## Compute the gradient

```

fprintf('Estimating the Gradient ... ');
estimated_grad = cell(2^pdim,2^pdim);
for x = 1:2^pdim
    for y = 1:2^pdim
        estimated_grad{y,x} = zeros(4^sdim);
    end
end
for k = 1:n
    estimated_grad{Y(k)+1,X(k)+1} = estimated_grad{Y(k)+1,X(k)+1} + RHO(:,k)*SIGMA(k+1,:)/(SIGMA(k+1,:)*RHO(:,k+1)*RHO_balancer(k+1));
end
for x = 1:2^pdim
    for y = 1:2^pdim
        estimated_grad{y,x} = -estimated_grad{y,x}/n*log2(exp(1));
    end
end
clear('k','x','y');
disp('Done. ');

```

Sanity check

```

induced_dev = 0;
for x = 1:2^pdim
    for y = 1:2^pdim
        induced_dev = induced_dev + trace(estimated_grad{y,x}*D{y,x});
    end
end
fprintf('<grad|D> = %f\n', induced_dev);
clear('x','y');

```

## Save the result to a file

```

save(['main_q(', char(datetime('now','Format','yyyy-MM-dd'T' 'HHmmss')), ').mat']);

```
