# Supplementary material for: Bounding and Estimating the Classical Information Rate of Quantum Channels with Memory
Source: arXiv:1903.00199 ancillary file (2020-02-17)
Supplement: Supplementary file 5 [file main_qgd.pdf]

# QSCs: Optimizing $\Delta(\hat{W})$ using modified gradient descent algorithm

\*This script requires user defined function db2mag.m

\*In this script, we propose an algorithm in minimizing  $\Delta(\hat{W})$ . This algorithm is based on:

1. The idea of the gradient descent algorithm
2. The 'alternative' method in estimating the directional derivative as listed in main\_q.mlx.

```
clear;clc;rng('shuffle');  
global REINDEX
```

## Configuration

# of consecutive channel usage to be simulated:

```
n = 1e5;
```

# of qubits in the memory/state system, the principle/input/output system, and the environment system:

```
sdim = 2;  
pdim = 1;  
envdim = 1;
```

Input distribution

```
Qx = ones(1,2^pdim);  
Qx = Qx./sum(Qx(:));
```

Channel parameters:

```
p_good = 0.95;  
p_bad = 0.1;  
load('H2_2.mat','H');% Requires sdim = 2
```

Step size and the limit on the number of steps in the gradient descent algorithm:

```
gamma = 1;  
gd_limit = 1000;
```

## Initialization

Standard Classical-to-Quantum modulation:

$$x \mapsto |x\rangle\langle x|.$$

```
C2Q = cell(1,2^pdim);  
for x = 1:2^pdim  
    temp = zeros(2^pdim,1);  
    temp(x) = 1;  
    C2Q{x} = temp;  
end  
clear('x','temp');
```

Standard partial measurement setup:

$$M_y := I_S \otimes |y\rangle\langle y|.$$

```
M = cell(1,2^pdim);  
for y = 1:2^pdim  
    temp = zeros(2^pdim);  
    temp(y,y) = 1;  
    M{y} = tensor(eye(2^sdim),temp);  
end  
clear('y','temp');
```

Generate a quantum GE channel (require pdim = 1)

```
AF = cell(1,2);  
AF{1} = diag([sqrt(p_good),sqrt(p_good),sqrt(p_bad),sqrt(p_bad)]);  
AF{1} = tensor(eye(2^(sdim-1)),AF{1});  
AF{2} = [0, sqrt(1-p_good), 0, 0;...  
        sqrt(1-p_good), 0, 0, 0;...  
        0, 0, 0, sqrt(1-p_bad);...  
        0, 0, sqrt(1-p_bad), 0];  
AF{2} = tensor(eye(2^(sdim-1)),AF{2});  
Us = tensor(expm(-1.2i*H),eye(2^pdim));  
AF{1} = Us*AF{1};  
AF{2} = Us*AF{2};  
W = matrix_QSC(AF,C2Q,M);  
%W = matrix_QSC(unitary2Qop(randU(2^(pdim+sdim+envdim)),envdim),C2Q,M);  
QW = cell(2^pdim,1);  
for y = 1:2^pdim  
    temp = zeros(size(W{1}));  
    for x = 1:2^pdim  
        temp = temp + W{y,x}.*Qx(x);
```

```

end
QW{y} = temp;
end
clear('x','y','temp','AF','Us','H');

```

Preallocation:

```

lambda_y = ones(1,n);
lambda_x = ones(1,n);
lambda_xy = ones(1,n);

```

Fast conversion between  $W(s, s_p; \bar{s}, \bar{s}_p)$  and  $W(s, \bar{s}; s_p, \bar{s}_p)$  format:

$$\text{REINDEX} \cdot [W(s, \bar{s}; s_p, \bar{s}_p)](:) = [W(s, s_p; \bar{s}, \bar{s}_p)](:)$$

$$\text{REINDEX}^T \cdot [W(s, s_p; \bar{s}, \bar{s}_p)](:) = [W(s, \bar{s}; s_p, \bar{s}_p)](:)$$

```

REINDEX = zeros(16^sdim);
for i = 1:4^sdim
    for j = 1:4^sdim
        A = zeros(4^sdim);
        A(i,j) = 1;
        B = zeros(size(A));
        size_S = 2^sdim;
        for sp1 = 1:size_S
            for sp2=1:size_S
                rho = zeros(size_S);
                rho(sp1,sp2) = 1;
                index = (1:size_S^2)*rho(:);
                sigma = zeros(size_S);
                for s1 = 1:size_S
                    for s2 = 1:size_S
                        sigma(s1,s2) = A(size_S*(s1-1)+sp1,size_S*(s2-1)+sp2);
                    end
                end
                B(:,index) = sigma(:);
            end
        end
        REINDEX(:,(1:16^sdim)*A(:)) = B(:);
    end
end
clear('A','B','size_S','rho','sigma','sp1','sp2','s1','s2','index','i','j');

```

Basis of the tangent space

```
[BASIS,basis] = base_of_change( 2^pdim, 2^pdim, sdim );
```

Create a CVX program which find a nearest QSC for a given input

```

initialize_CVX_psd( 'main_qgd_cvx_psd.m', sdim, pdim,'matrix_W');
initialize_CVX_grad( 'main_qgd_cvx_grad.m', sdim, pdim);

```

## Simulate Channle Input $X_1^n$ /Output $Y_1^n$ process

```

fprintf('Simulating channel with %d binary i/o ... ', n);
X = randi(2,1,n)-1;
Y = zeros(size(X));
rho = eye(2^sdim)/2^sdim; rho = rho(:);
one = eye(2^sdim); one = one(:);
L = transpose(tril(ones(2^pdim)));
for k = 1:n
    PMF = zeros(1,2^pdim);
    for y = 1:2^pdim
        PMF(y) = dot(W{y,X(k)+1}*rho,one);
    end
    CDF = PMF*L;
    Y(k) = sum(rand > CDF);
    rho = W{Y(k)+1,X(k)+1}*rho;
    rho = rho./dot(one,rho);
end
disp('Done. ');
clear('rho','one','PMF','CDF','L','k','y');

```

Using Forward Message Passing Method w.r.t the actual QSC  $W$  to estimate  $\frac{1}{n} H(Y_1^n | X_1^n)$

```

fprintf('Estimating H(Y|X) ... ');
rho = eye(2^sdim)/2^sdim; rho = rho(:);
one = eye(2^sdim); one = one(:);
for k = 1:n
    rho = W{Y(k)+1,X(k)+1}*rho;
    lambda_xy(k) = dot(one,rho);
    rho = rho./lambda_xy(k);
end
hY_given_X = -sum(log2(lambda_xy))/n;
fprintf(' = %f\n', hY_given_X);

```

```
clear('rho','one','k');
```

Using Forward Message Passing Method w.r.t the actual QSC  $W$  to estimate  $\frac{1}{n} H(Y_1^n)$

```
fprintf('Estimating H(Y) ... ');
rho = eye(2^sdim)/2^sdim; rho = rho(:);
one = eye(2^sdim); one = one(:);
for k = 1:n
    rho = QW{Y(k)+1}*rho;
    lambda_y(k) = dot(one,rho);
    rho = rho./lambda_y(k);
end
hY = -sum(log2(lambda_y))/n;
fprintf(' = %f\n', hY);
clear('rho','one','k');
```

### Information Rate

```
I = hY - hY_given_X;
fprintf('Information rate = %f\n', I);
```

### Setup an initial AF-QSC $\hat{W}$

```
W = matrix_QSC(unitary2Qop(randU(2^(pdim+sdim+envdim)),envdim),C2Q,M);
if ~isQSC(W,REINDEX)
    disp('The AUX channel is not QSC!!!');
end
clear('QW');
```

### Gradient Descent Method

```
gd_time = zeros(1,gd_limit+1);
gd_time(1) = 0;
gd_W_List = cell(1,gd_limit+1);
gd_W_List{1} = W;
gd_status = ones(1,gd_limit+1);
tic;
f = waitbar(0,'The gradient descent method ... ');
for gd_counter = 1:gd_limit
```

Forward pass:

```
waitbar((gd_counter-1)/gd_limit, f,...
    sprintf(['%d Forward pass ... ', gd_counter]));
rho = eye(2^sdim)/2^sdim;
RHO = zeros(4^sdim,n+1);
RHO(:,1) = rho(:);
RHO_balancer = ones(1,n+1);
one = eye(2^sdim); one = one(:);
for k = 1:n
    RHO(:,k+1) = W{Y(k)+1,X(k)+1}*RHO(:,k);
    RHO_balancer(k+1) = dot(one,RHO(:,k+1));
    RHO(:,k+1) = RHO(:,k+1)./RHO_balancer(k+1);
end
clear('rho','k','one');
```

Backward pass:

```
waitbar((gd_counter-0.75)/gd_limit, f,...
    sprintf(['%d Backward pass ... ', gd_counter]));
sigma = eye(2^sdim);
rSIGMA = zeros(4^sdim, n+1);
rSIGMA(:,1) = sigma(:);
rSIGMA_balancer = ones(1,n+1);
one = eye(2^sdim); one = one(:);
trans_W = cell(size(W));
for k = 1: numel(W)
    trans_W{k} = transpose(W{k});
end
for k = 1:n
    rSIGMA(:,k+1) = trans_W{Y(n-k+1)+1,X(n-k+1)+1}*rSIGMA(:,k);
    rSIGMA_balancer(k+1) = dot(one,rSIGMA(:,k+1));
    rSIGMA(:,k+1) = rSIGMA(:,k+1)./rSIGMA_balancer(k+1);
end
SIGMA = zeros(n+1,4^sdim);
SIGMA_balancer = ones(n+1,1);
for k = 1:n+1
    SIGMA(k,:) = transpose(rSIGMA(:,n+2-k));
    SIGMA_balancer(k) = rSIGMA_balancer(n+2-k);
end
clear('trans_W','sigma','k','one','rSIGMA','rSIGMA_balancer');
```

Compute the gradient:

```
waitbar((gd_counter-0.5)/gd_limit,f,...
```

```

    sprintf(['%d] Estimate gradient ... ', gd_counter));
estimated_grad = cell(2^pdim,2^pdim);
for x = 1:2^pdim
    for y = 1:2^pdim
        estimated_grad{y,x} = zeros(4^sdim);
    end
end
for k = 1:n
    estimated_grad{Y(k)+1,X(k)+1} = estimated_grad{Y(k)+1,X(k)+1} + RHO(:,k)*SIGMA(k+1,:)/(SIGMA(k+1,:)*RHO(:,k+1)*RHO
end
for x = 1:2^pdim
    for y = 1:2^pdim
        estimated_grad{y,x} = -estimated_grad{y,x}/n*log2(exp(1));
    end
end
clear('k','x','y');

```

Project the gradient onto the subspace defined as

$$T := \left\{ D^{y|x} : \mathcal{D}(\mathcal{H}_S) \rightarrow \mathcal{D}(\mathcal{H}_S) \mid D^{y|x} \text{ is linear, and } \text{tr} \left( \sum_y D^{y|x}(\rho) \right) = 0 \ \forall \rho \right\}$$

```

projected_grad = zeros(1,size(basis,3));
for k = 1:size(basis,3)
    D = basis(:, :, k);
    for x = 1:2^pdim
        for y = 1:2^pdim
            projected_grad(k) = projected_grad(k) + trace(estimated_grad{y,x}*D{y,x});
        end
    end
end
for x = 1:2^pdim
    for y = 1:2^pdim
        estimated_grad{y,x} = zeros(4^sdim);
        for k = 1:size(basis,3)
            D = basis(:, :, k);
            estimated_grad{y,x} = estimated_grad{y,x} + projected_grad(k).*D{y,x};
        end
    end
end
clear('k','D','x','y','projected_grad');

```

Apply the changes

```

waitbar((gd_counter-0.2)/gd_limit,f,...
    sprintf(['%d] Gradient descent ... ', gd_counter));
W_0 = W;
for x = 1:2^pdim
    for y = 1:2^pdim
        W{y,x} = W{y,x} - gamma*estimated_grad{y,x};
    end
end
W_1 = W;

```

Project back to the domain of QSCs using cvx

Following requirements have to be satisfied:

1.  $W^{y|x}(s, s_p; \bar{s}, \bar{s}_p)$  must be a PSD matrix;
2.  $\sum_{s=\bar{s}} W^{y|x}(s, s_p; \bar{s}, \bar{s}_p) = \delta(s_p, \bar{s}_p)$ .

```

waitbar((gd_counter-0.15)/gd_limit,f,...
    sprintf(['%d] Project to the nearest QSC ... ', gd_counter))
% Convert the pseudo_QSC into (s,sp;s',sp';y,x) format
Q = zeros(4^sdim,4^sdim,2^pdim,2^pdim);
for y = 1:2^pdim
    for x = 1:2^pdim
        temp_B = W{y,x};
        temp_A = zeros(size(temp_B));
        temp_A(:) = transpose(REINDEX)*temp_B(:);
        Q(:, :, y, x) = temp_A;
    end
end
% Run the CVX program (Q, matrix_W)
main_qgd_cvx_psd;
matrix_W = Q;
%cvx_status = 'disabled';
% Convert matrix_W back to the proper format
W = cell(2^pdim);
for y = 1:2^pdim
    for x = 1:2^pdim
        temp_A = matrix_W(:, :, y, x);
        temp_B = zeros(size(temp_A));
        temp_B(:) = REINDEX*temp_A(:);
        W{y,x} = temp_B;
    end
end

```

```

d1 = 0;
for x = 1:2^pdim
    for y = 1:2^pdim
        d1 = d1 + norm((W_1{y,x} - W_0{y,x}), 'fro')^2;
    end
end
d2 = 0;
for x = 1:2^pdim
    for y = 1:2^pdim
        d2 = d2 + norm((W{y,x} - W_1{y,x}), 'fro')^2;
    end
end
d3 = 0;
for x = 1:2^pdim
    for y = 1:2^pdim
        d3 = d3 + norm((W{y,x} - W_0{y,x}), 'fro')^2;
    end
end
if strcmp(cvx_status, 'Solved')
    gd_status(gd_counter+1) = 1;
else
    gd_status(gd_counter+1) = 0;
end
if isQSC(W, REINDEX)
    fprintf(['%d: %s] Projection W0 -- %f --> W0+grad -- %f --> W1 (-- %f -->)\n', ...
            gd_counter, cvx_status, sqrt(d1), sqrt(d2), sqrt(d3));
else
    fprintf(['*%d: %s] Projection W0 -- %f --> W0+grad -- %f --> W1 (-- %f -->)\n', ...
            gd_counter, cvx_status, sqrt(d1), sqrt(d2), sqrt(d3));
end

clear('cvx_cputime', 'cvx_optbnd', 'cvx_optval', 'cvx_slvitr', 'cvx_slvtol', 'cvx_status', 'matrix_W');
clear('Q', 'x', 'y', 'temp_A', 'temp_B', 'matrix_W', 'd1', 'd2', 'd3');

```

Wrap-up:

```

gd_W_List{gd_counter+1} = W;
gd_time(gd_counter+1) = toc;
end
close(f);
clear('gd_counter', 'f');

```

## Post processing for the GDA

For each  $\hat{W}$ , estimate  $\frac{1}{n}H(Y_1^n)$ , and compute  $\bar{I}(\hat{W})$ ,  $\underline{I}(\hat{W})$  and  $\Delta(\hat{W})$ .

```

fprintf('Gathering the data for the gradient descent method ... ');
f = waitbar(0, 'Post-processing for the gradient method ... ');
gd_upper_hY_List = zeros(1, gd_limit+1);
gd_aux_hXY_List = zeros(1, gd_limit+1);
for gd_counter = 1:gd_limit+1
    W = gd_W_List{gd_counter};
    QW = cell(2^pdim, 1);
    for y = 1:2^pdim
        temp = zeros(size(W{1}));
        for x = 1:2^pdim
            temp = temp + W{y,x}.*Qx(x);
        end
        QW{y} = temp;
    end
    clear('temp', 'x', 'y');
    % 1/n * H(Y1, ..., Yn)
    rho = eye(2^sdim)/2^sdim; rho = rho(:);
    one = eye(2^sdim); one = one(:);
    for k = 1:n
        rho = QW{Y(k)+1} * rho;
        lambda_y(k) = dot(one, rho);
        rho = rho ./ lambda_y(k);
    end
    clear('rho', 'one', 'k');
    gd_upper_hY_List(gd_counter) = -sum(log2(lambda_y))/n;
    % 1/n * H(Y1, ..., Yn | X1, ..., Xn)
    rho = eye(2^sdim)/2^sdim; rho = rho(:);
    one = eye(2^sdim); one = one(:);
    for k = 1:n
        rho = W{Y(k)+1, X(k)+1} * rho;
        lambda_xy(k) = dot(one, rho);
        rho = rho ./ lambda_xy(k);
    end
    clear('rho', 'one', 'k');
    gd_aux_hXY_List(gd_counter) = -sum(log2(lambda_xy))/n;
    waitbar(gd_counter/(gd_limit+1), f);
end
close(f);
clear('f', 'gd_counter');
gd_IR_L = gd_upper_hY_List - gd_aux_hXY_List;
gd_IR_U = gd_upper_hY_List - hY_given_X;

```

```
gd_GAP = gd_IR_U - gd_IR_L;
disp('Done.');
```

## Plot

```
hold on;
plot(gd_time,gd_IR_L,'b');
plot(gd_time,gd_IR_U,'r');
%plot(em_time,em_IR_L,'b--');
%plot(em_time,em_IR_U,'r--');
plot([0,max(gd_time)],ones(1,2)*I,'k--');%plot([0,max([gd_time,em_time])],ones(1,2)*I,'k--');
hold off;
legend('GD:IRLB','GD:IRUB','IR');
title(sprintf('Gradient Descent Method with "CVX drag-back" in each step'));
xlabel('Time/seconds');
ylabel('bits/channel use');
xlim([0,gd_time(gd_limit+1)]);
```

## Save the result to a file

```
save(['main_qgd(',char(datetime('now','Format','yyyy-MM-dd'T'HHmmss)),')'.mat']);
```
